# Supplementary material for: Prepare Lighter and Faster for Open-Vocabulary Queries: A Query-Wise 3D Segmenter for Gaussian Splatting
Source: arXiv:2611.19429 source file (2026-11-14)
Supplement: Supplementary file 1 [file X_suppl.tex]

% \clearpage
\setcounter{page}{1}
% \maketitlesupplementary


\begin{abstract}
    This supplementary material provides the following:

    1) Implementation details.

    2) More Ablation Study.

    3) Runtime Analysis.

    4) Additional quantitative and qualitative results on LERF-OVS, 3D-OVS, and ScanNet. 

    5) Scalability to Large Scenes.

    6) Limitations and Future Works.



We also include a supplementary video for more visual results. 
\end{abstract}

\section{Implementation Details}
All experiments are conducted on a single NVIDIA A100 40GB GPU. Image-wise dense CLIP features are extracted using ProxyCLIP \cite{proxyclip} with the CLIP-B/16 backbone and DINO-v2. Tracking and segmentation are benchmarked using HQ-SAM 2 \cite{samhq} and EfficientTAM \cite{efficienttam}. A \emph{single} config (similarity threshold $\tau{=}0.75$, minimum area constraint $A_{\min}{=}10$) is used across all benchmarks with no per-dataset tuning. Frame budget $P$'s trade-off is discussed in Tab.~8/Fig.~5 of the main paper. All choices are empirically validated.

\subsection{Visualization of the method breakdown.}
We provide qualitative visualizations of several key components of our method in \cref{fig:pivot_comparison}, including visibility voting, multi-instance localization, and mask refinement, to complement the descriptions in the main paper.

\begin{figure}[t!]
    \centering

    \begin{subfigure}{\columnwidth}
        \centering
        \includegraphics[width=\columnwidth]{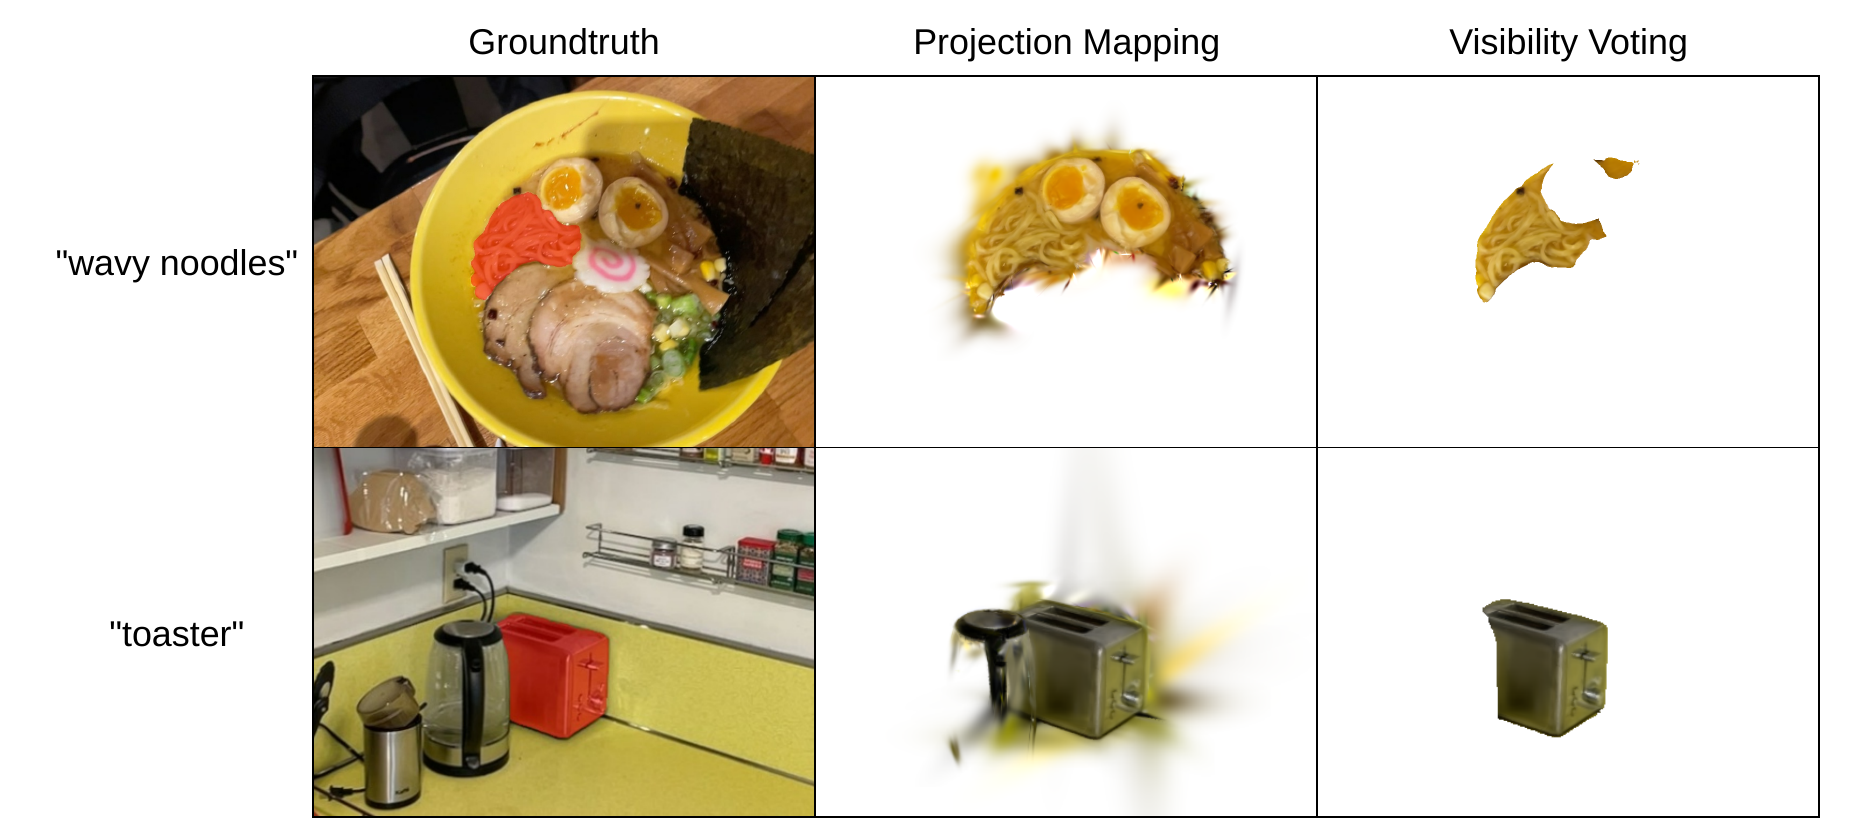}
        \caption{
        Comparison between projection mapping and the proposed visibility voting.
        }
        \label{fig:8-voting}
    \end{subfigure}

    \vspace{4pt}

    \begin{subfigure}{\columnwidth}
        \centering
        \includegraphics[width=.9\linewidth]{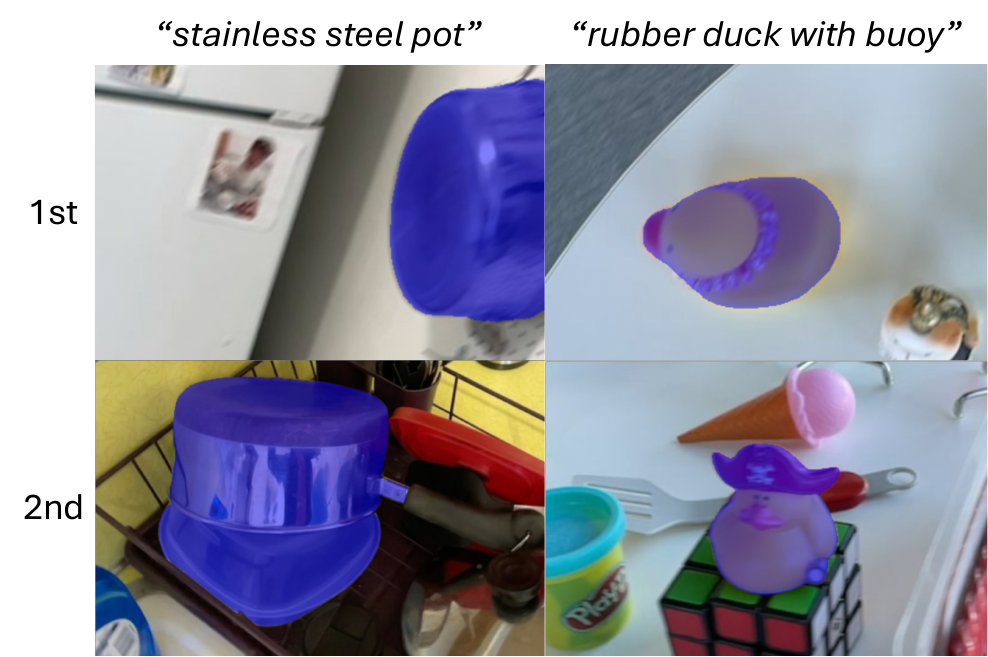}
        \caption{Multi-instance pivot localization.}
        \label{fig:5-multi-instance}
    \end{subfigure}

    \vspace{4pt}

    \begin{subfigure}{\columnwidth}
        \centering
        \includegraphics[width=\linewidth]{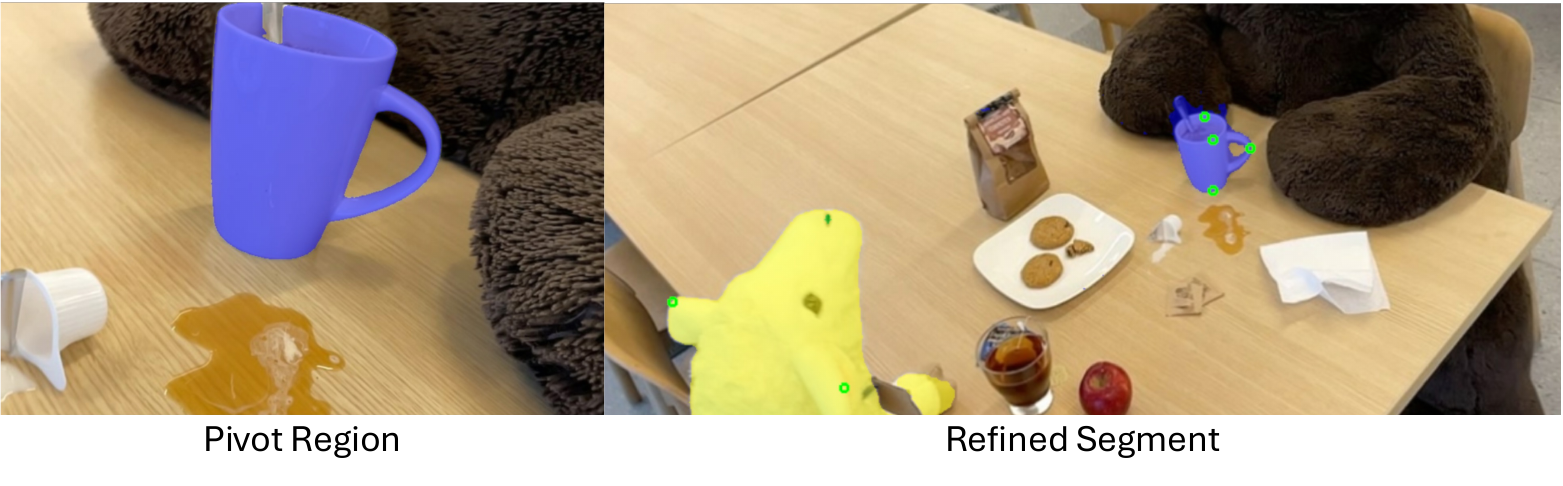}
        \caption{Mask refinement for the query ``coffee mug''. Left: pivot region in the pivot view. Right: refined segment after tracklet refinement. Blue indicates the newly chosen segment, yellow the eliminated misaligned segment, and green circles show FPS point prompts used for refinement.}
        \label{fig:4-mask_refine}
    \end{subfigure}

    \caption{\textbf{Visualization of the method breakdown.}}
    \label{fig:pivot_comparison}
\end{figure}

\subsection{2D Pivot Region Localization Algorithm}
We provide the pseudo code for 2D instance localization (Section 3.1 in the main paper). The pseudo code details how we localize and extract pivot regions from the cosine similarity maps.


\begin{algorithm}
\caption{Extract Pivot Region of Prompted Query}
\label{alg:extract-one-region}
\begin{algorithmic}[1]
\REQUIRE Similarity maps $\mathbf{S} \in \mathbb{R}^{N \times H \times W}$, threshold $\tau$, minimum area $A_{\min}$
\ENSURE Single region $(\mathbf{R}, i, s, a)$ or \textbf{None}
\STATE $(s_{\max}, (i, p)) \gets \arg\max \mathbf{S}$ \hfill // highest similarity
\IF{$s_{\max} < \tau$}
    \RETURN \textbf{None}
\ENDIF
\STATE $\mathbf{T}_i \gets [\mathbf{S}_i \ge \tau]$ \hfill // thresholded map
\STATE $\mathbf{R} \gets \text{ConvFloodFill}(\mathbf{T}_i, p)$ \hfill // extracted region
\STATE $\mathbf{R} \gets \text{ConvMorphErosion}(\mathbf{R})$ \hfill // refine boundary
\STATE $s \gets \frac{\sum (\mathbf{S}_i \odot \mathbf{R})}{a}$
\STATE $a \gets \sum \mathbf{R}$ \hfill // check region area
\IF{$a < A_{\min}$}
    \RETURN \textbf{None}
\ENDIF
\RETURN $(\mathbf{R}, i, s, a)$
\end{algorithmic}
\end{algorithm}

\begin{algorithm}[t]
\caption{Convolutional Flood Fill via Convolutional Expansion}
\label{alg:conv-flood-fill}
\begin{algorithmic}[1]
\REQUIRE Binary mask $\mathbf{B} \in \{0,1\}^{H \times W}$, seed pixel $p=(y,x)$
\ENSURE Connected region mask $\mathbf{R} \in \{0,1\}^{H \times W}$

\STATE Initialize region mask $\mathbf{R} \gets \mathbf{0}_{H\times W}$
\STATE $\mathbf{R}[y,x] \gets 1$
\STATE Define $3\times3$ kernel $\mathbf{K} \gets \mathbf{1}_{3\times3}$

\REPEAT
    \STATE $\mathbf{E} \gets (\text{Conv2D}(\mathbf{R}, \mathbf{K}, \text{padding}=1) > 0)$
    \STATE $\mathbf{R}_{new} \gets \mathbf{E} \land \mathbf{B}$
\UNTIL{$\sum \mathbf{R}_{new} = \sum \mathbf{R}$}

\STATE $\mathbf{R} \gets \mathbf{R}_{new}$
\RETURN $\mathbf{R}$

\end{algorithmic}
\end{algorithm}

\begin{algorithm}[t]
\caption{Convolutional Morphological Erosion for Boundary Cropping}
\label{alg:conv-morph-erosion}
\begin{algorithmic}[1]
\REQUIRE Binary mask $\mathbf{M} \in \{0,1\}^{H \times W}$, edge margin $m$
\ENSURE Eroded mask $\mathbf{R}$

\STATE $k \gets 2m + 1$ \hfill // kernel size
\STATE $\mathbf{M}_{inv} \gets 1 - \mathbf{M}$ \hfill // invert mask

\STATE $\mathbf{E}_{inv} \gets \text{MaxPool2D}(\mathbf{M}_{inv}, k, \text{stride}=1, \text{padding}=m)$

\STATE $\mathbf{R} \gets 1 - \mathbf{E}_{inv}$ \hfill // invert back

\RETURN $\mathbf{R}$
\end{algorithmic}
\end{algorithm}

We select the pivot mask using ProxyCLIP~\cite{proxyclip}, which aggregates semantic evidence across all pixels from all views rather than relying on a single-view prediction. This global reasoning significantly increases the likelihood of identifying a correct and representative pivot region, as the model can exploit multi-view semantic consistency while suppressing noisy local responses. 

Empirically, the robustness of this step is reflected in the performance of our 2D localization module, which achieves \textbf{93\% accuracy on LERF-OVS} and \textbf{100\% on 3D-OVS}. These results indicate that the pivot selection succeeds in the vast majority of cases and provides a reliable initialization for the subsequent 3D segmentation stage. In practice, we rarely observe failures where the pivot mask does not overlap with the queried object. In the rare case where the pivot cannot be identified, the framework can flexibly fall back to a stronger vision-language grounding model (e.g., Grounded-SAM~\cite{groundedsam}) to reinitialize a more accurate pivot region, preventing catastrophic failure in downstream applications.

\myheading{Visualization of extracted instance Gaussians}
To further evaluate the quality of our visibility voting mechanism, we visualize renderings of the extracted instance Gaussians without foreground/background blending. As shown in \Cref{fig:instance-gaussians}, the selected Gaussians form coherent 3D object representations that accurately capture the spatial extent and geometric structure of the queried instances. The clean foreground--background separation and preserved object geometry demonstrate that visibility voting effectively aggregates multi-view evidence while suppressing spurious Gaussian assignments.
{\begin{figure}[ht!]
    \centering
    \includegraphics[width=\linewidth]{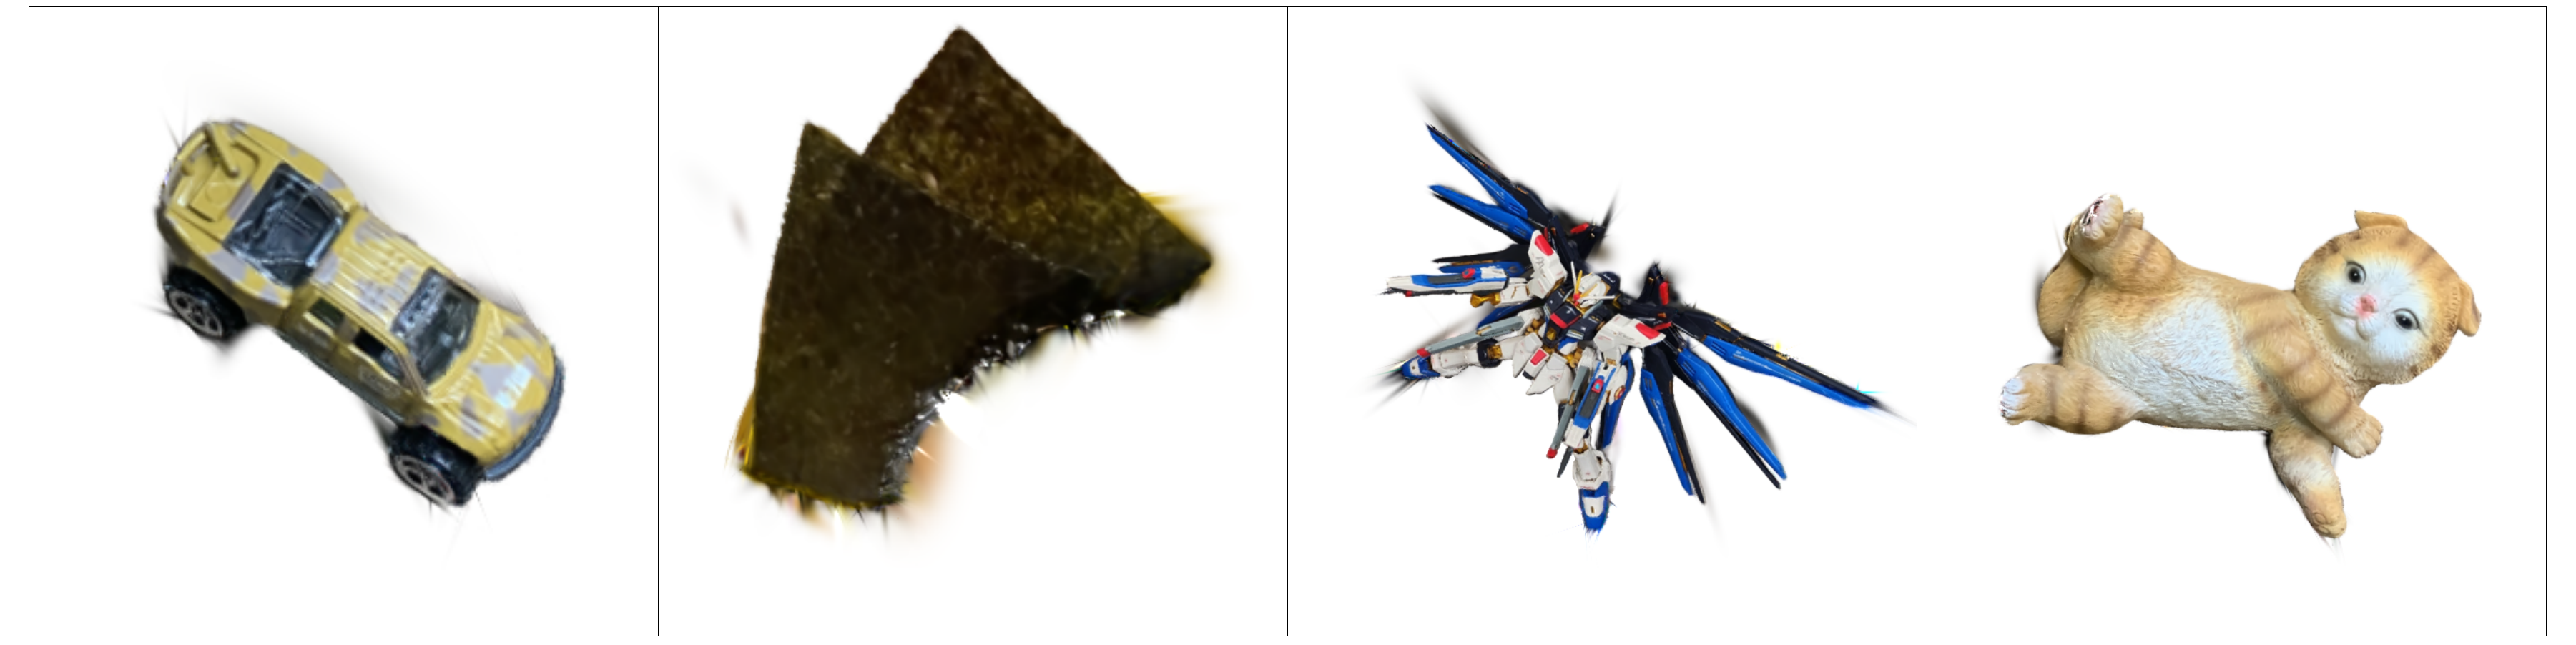}
    \vspace{-5pt}
    \caption{Visualization of instance Gaussians extracted by our visibility voting mechanism without foreground/background blending.}
    \vspace{-10pt}
\label{fig:instance-gaussians}
\end{figure}}

\myheading{Baseline for query-driven open-vocabulary 3D instance segmentation.}
Existing methods formulate open-vocabulary 3D understanding as either scene-level feature learning or instance-aware reconstruction, rather than query-driven 3D instance segmentation. As a result, no established baseline exists for our problem setting.

To enable a principled ablation study, we construct a simple three-stage baseline that follows the same query-driven formulation as our method while replacing each proposed component with a straightforward alternative. As illustrated in \cref{fig:baseline_pipeline}, the baseline consists of feature extraction, multi-view instance localization, and 3D lifting. For feature extraction, we first apply the automatic SAM mask generator to every input image and extract a mask-wise CLIP feature for each generated mask instead of our dense pixel-level CLIP representation. Given a text query, we compute the cosine similarity between the CLIP text embedding and the CLIP embedding of every candidate mask, and select the highest-scoring mask as the pivot region. We then propagate the pivot mask across views using HQ-SAM~2~\cite{samhq}. Finally, we construct the 3D instance by projection mapping, assigning each Gaussian to the instance if its projection falls within the propagated masks.


\begin{figure*}[ht!]
    \centering
    \vspace{-4pt}
    \includegraphics[width=\linewidth]{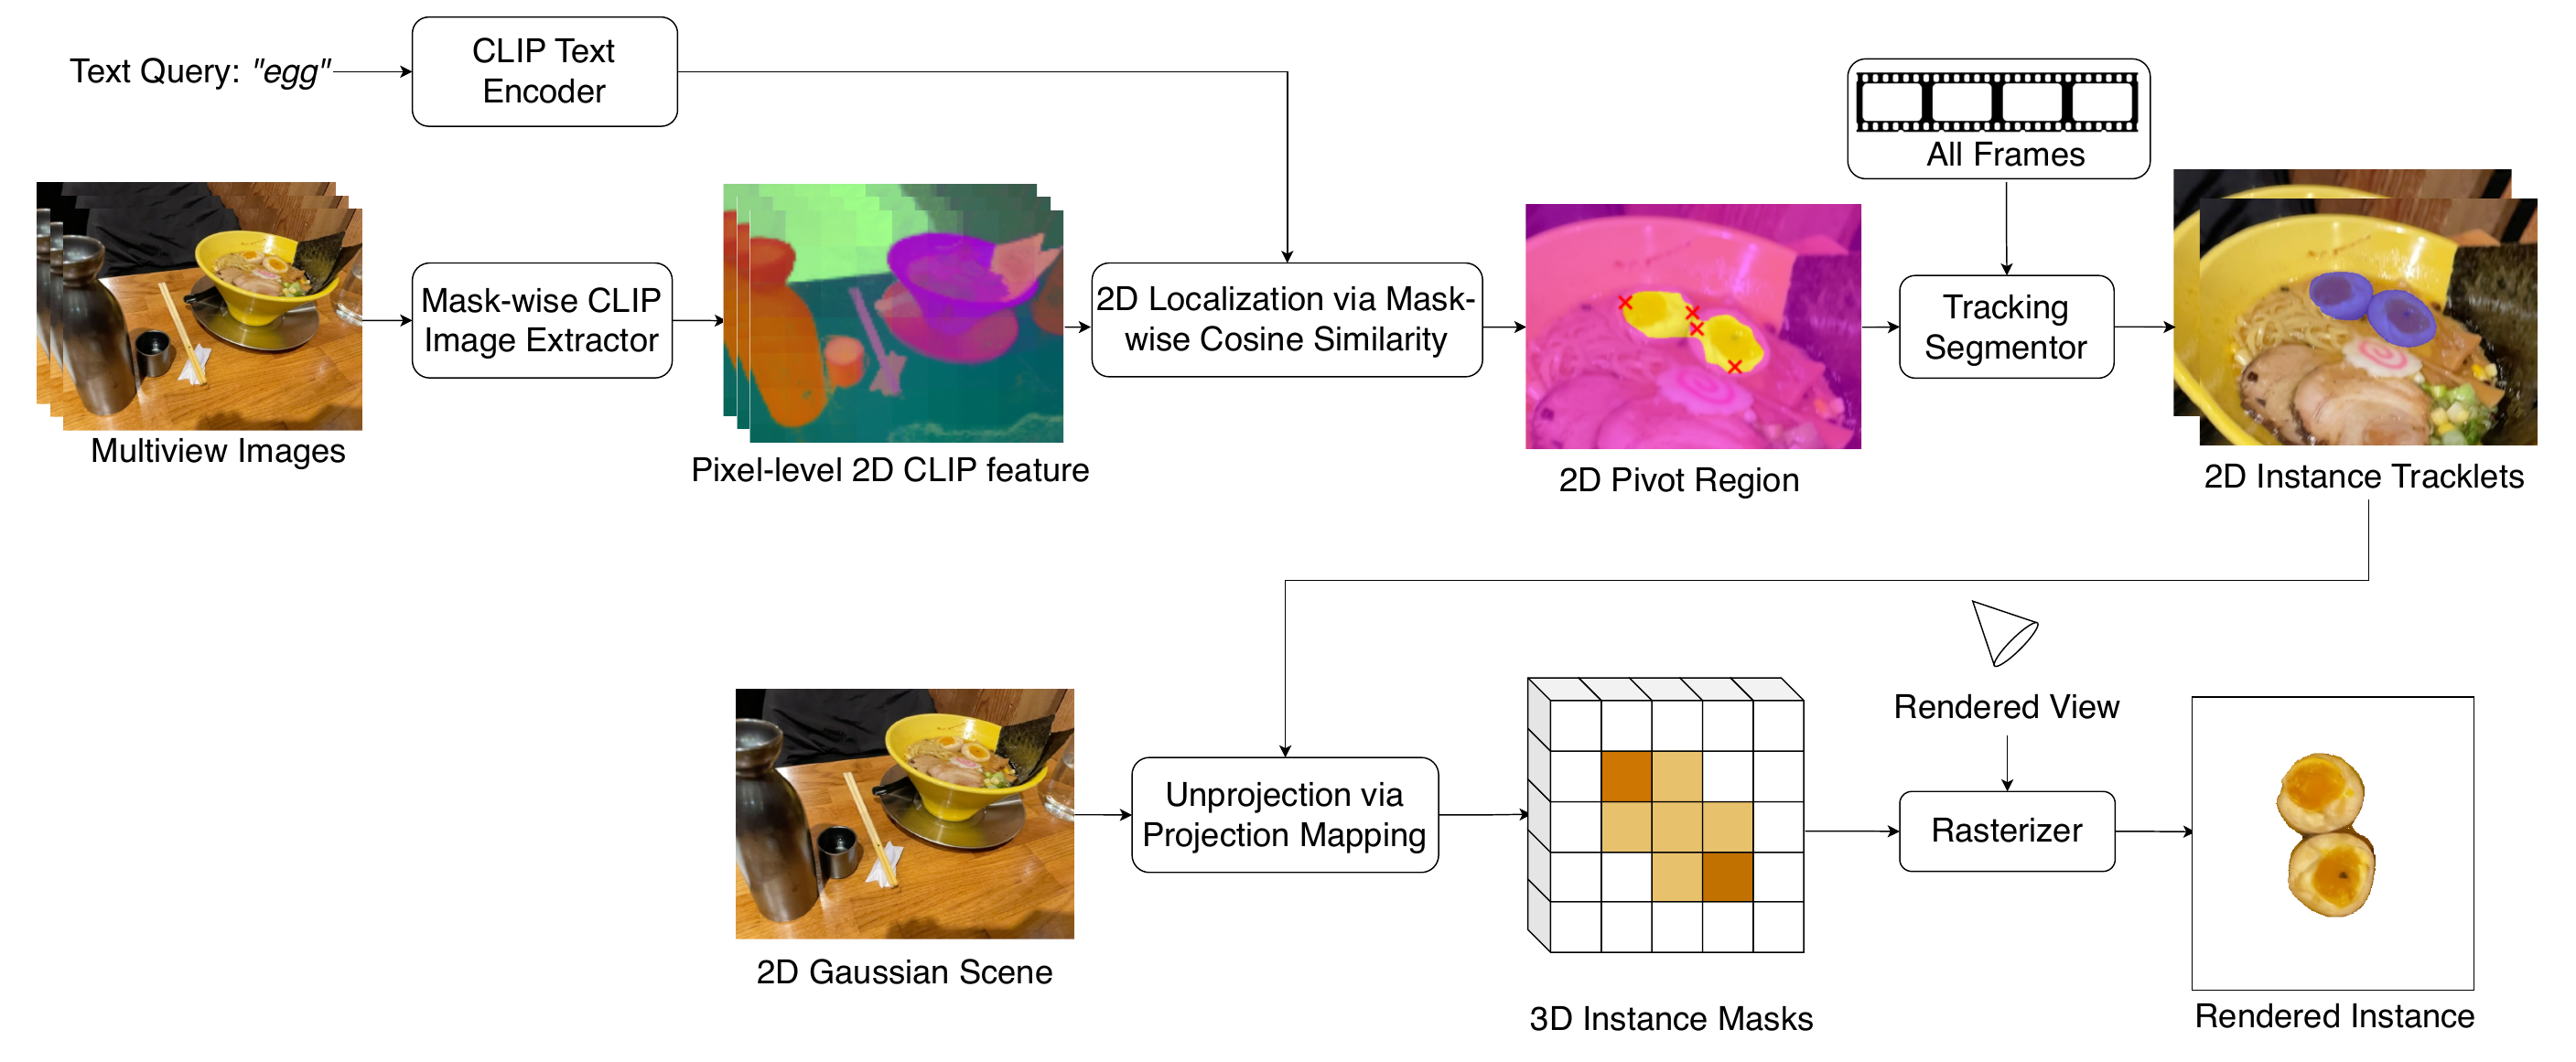}
    \vspace{-4pt}
    \caption{Baseline for query-driven open-vocabulary 3D instance segmentation.}
    \vspace{-2pt}
    \label{fig:baseline_pipeline}
\end{figure*}

\myheading{Pipeline for full-scene 3D evaluation.}
We extend our query-wise framework to full-scene understanding with only two lightweight modifications (highlighted in green in \Cref{fig:fullscene}) while preserving its core design and training-free nature. The main idea is to iteratively segment class-agnostic 3D instances and assign semantic features to their constituent Gaussians.

We first randomly select an unvisited Gaussian as the pivot Gaussian. To identify a reliable reference view, we rank all input views according to the visibility of the pivot Gaussian and its neighboring Gaussians with similar surface normals, while discarding Gaussians projected near the image boundary or viewed from the rear. We choose the highest-ranked view as the pivot view and use the CLIP feature at the projected pixel of the pivot Gaussian as the pivot feature. Similar to the query-wise pipeline, we compute the cosine similarity between the pivot feature and every pixel in the pivot view, then apply the proposed flood-fill algorithm to obtain the pivot region. We subsequently feed this pivot region into the same multi-view propagation and visibility-voting pipeline described in the main paper to construct the complete 3D instance mask.

After segmenting a 3D instance, we mark all its Gaussians as visited and repeat the above procedure until every Gaussian belongs to an instance. Finally, we average the CLIP embeddings of every pixels within the propagated tracklets of each instance and assign the resulting embedding to all Gaussians in that instance.

\begin{figure*}[t]
    \centering
    \vspace{-4pt}
    \includegraphics[width=\linewidth]{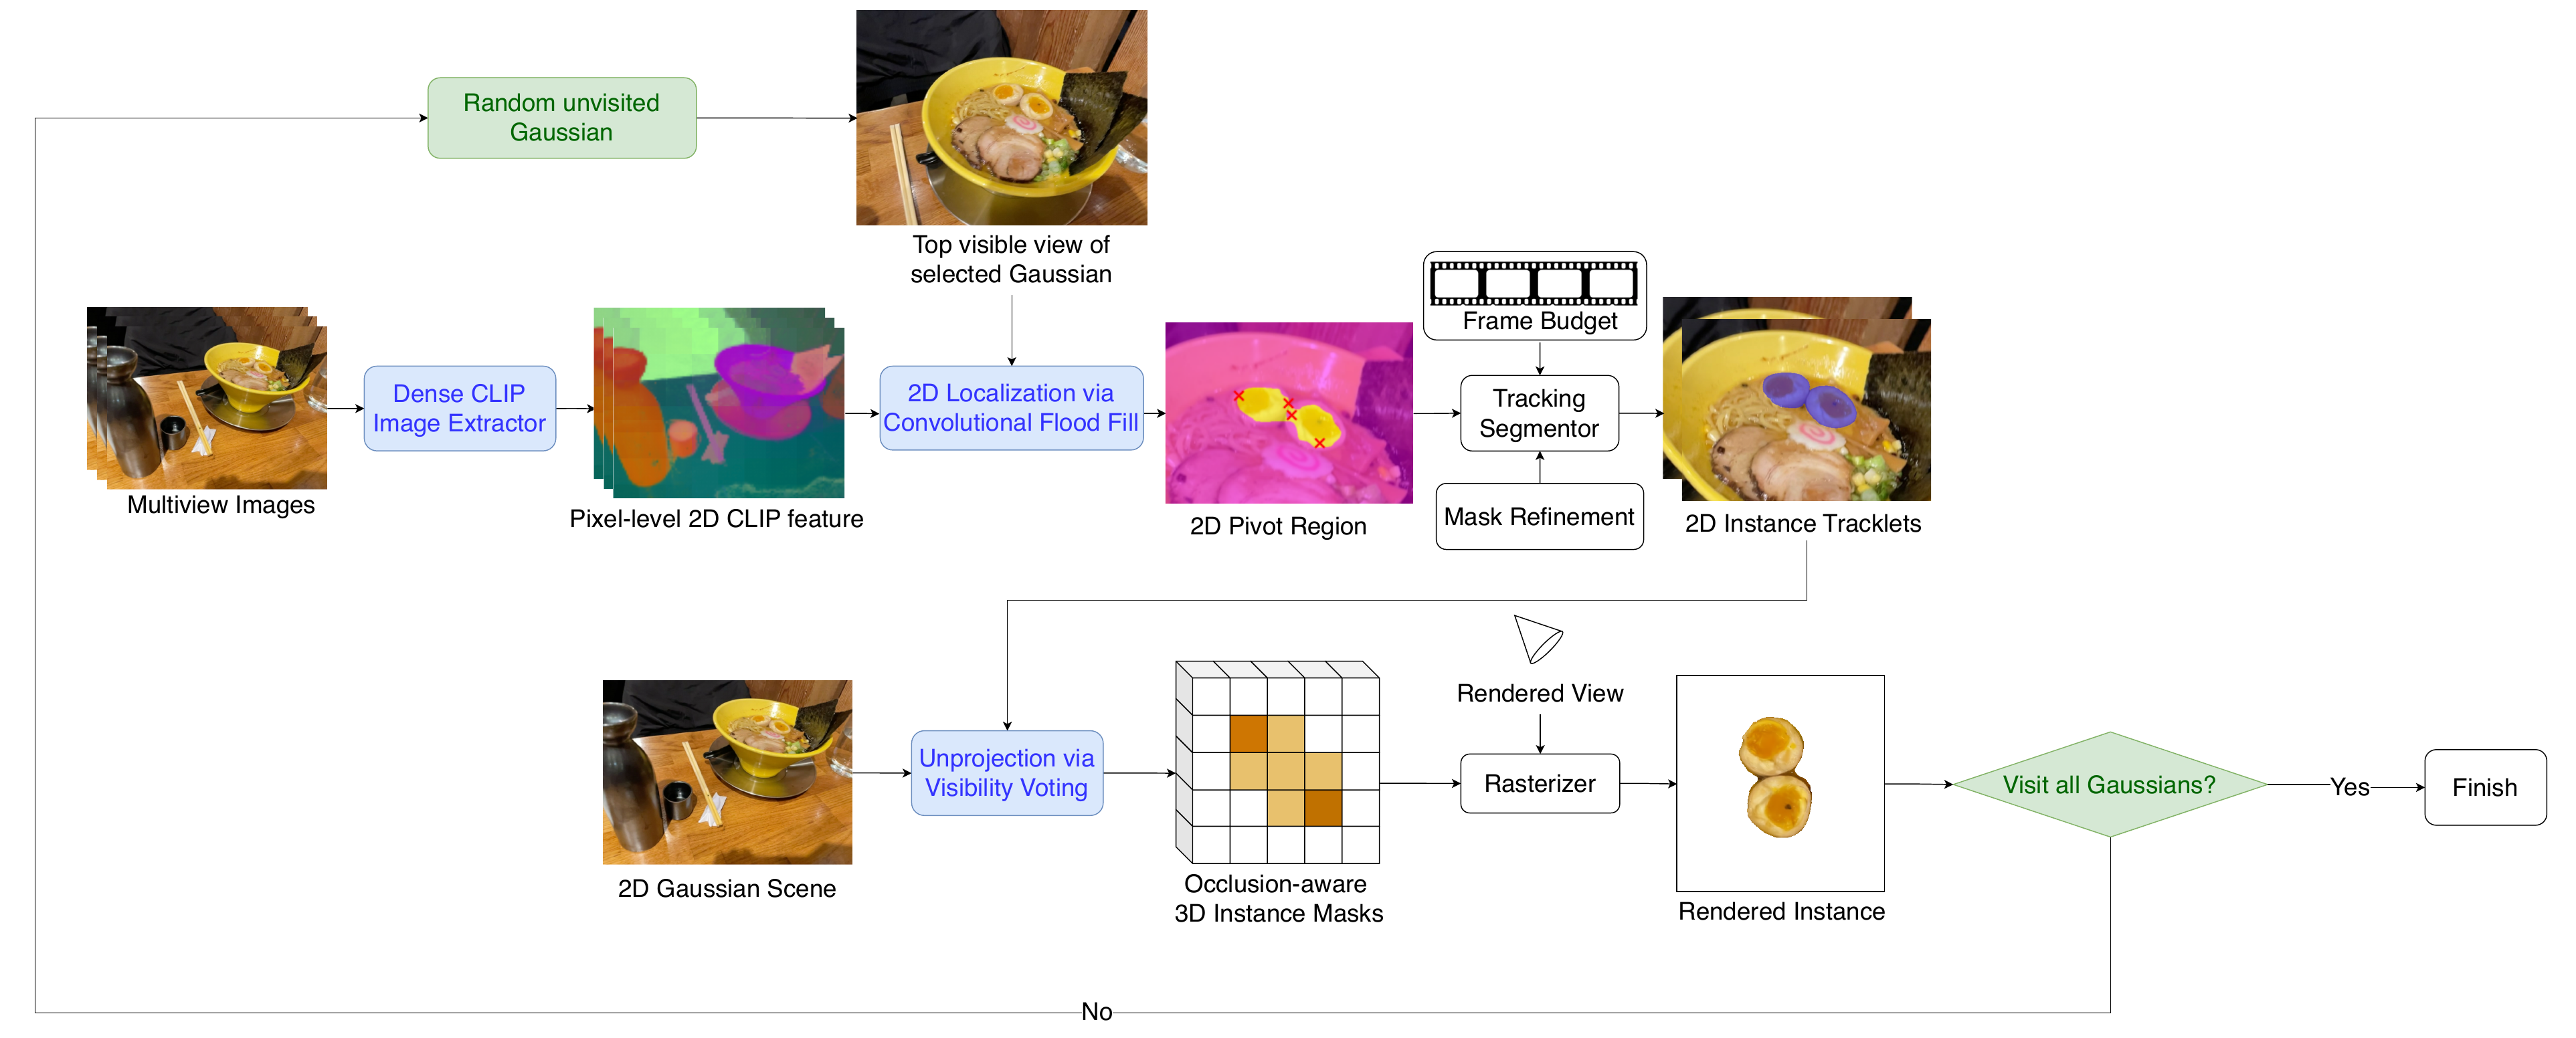}
    \vspace{-4pt}
    \caption{Pipeline for class-agnostic 3DIS evaluation.}
    \vspace{-2pt}
    \label{fig:fullscene}
\end{figure*}

\section{More Ablation Study}
\myheading{Effectiveness of different DINO features.}
We compare different DINO backbones on LERF‑OVS to assess their effect on open‑vocabulary 3D instance segmentation. As shown in \cref{tab:ablation_dino}, DINOv2~\cite{dinov2} achieves the best performance, clearly outperforming both DINO~\cite{dino} and DINOv3~\cite{dinov3}. This improvement comes from DINOv2’s stronger alignment between global semantics and local spatial features, leading to more reliable dense matching and more precise query localization. Although DINOv3 is competitive, its weaker mid‑level representations result in slightly lower accuracy for fine‑grained correspondence.

\begin{table}[t]
\caption{Performance comparison with different DINO backbones.}
\label{tab:ablation_dino}
\scriptsize
\centering
\setlength{\tabcolsep}{8pt}
\renewcommand{\arraystretch}{1.2}
\begin{tabular}{lcc}
\toprule
DINO version & mIoU $\uparrow$ & mAcc@0.25 $\uparrow$ \\
\midrule
DINO \cite{dino} & 56.90 & 43.49 \\
DINOv2 \cite{dinov2} & \textbf{63.02} & \textbf{81.91} \\
DINOv3 \cite{dinov3} & 60.41 & 74.65 \\
\bottomrule
\end{tabular}
\end{table}

\myheading{Ablation on the prompt-based mask refinement module.}
We further investigate the sensitivity of our prompt-based mask refinement module to the number of point prompts. As shown in Table~\ref{tab:point_prompt_ablation}, the performance remains relatively stable when varying the number of point prompts from 1 to 4, with mIoU ranging from 0.6030 to 0.6097 and mAcc@25 ranging from 0.7280 to 0.7359. Using 3 point prompts achieves the highest mIoU of 0.6097, while 4 point prompts yields the best mAcc@25 of 0.7359. Increasing the number of prompts to 5, however, leads to a noticeable drop in mAcc@25, suggesting that excessive prompts may introduce noisy or redundant guidance during refinement. Overall, these results demonstrate that the proposed refinement module is not highly sensitive to the number of point prompts and remains effective with a small number of prompts. In our experiments, we use 3 point prompts as a good trade-off between refinement effectiveness and prompt efficiency.
\begin{table}[t]
    \centering
    \caption{Ablation study on the number of point prompts used by the prompt-based mask refinement module on LERF-OVS~\cite{lerf}.}
    \label{tab:point_prompt_ablation}
    \begin{tabular}{c|cc}
        \toprule
        \textbf{Number of Point Prompts} & \textbf{mIoU $\uparrow$} & \textbf{mAcc@25 $\uparrow$} \\
        \midrule
        1 & 0.6030 & 0.7315 \\
        2 & 0.6030 & 0.7315 \\
        3 & \textbf{0.6095} & 0.7280 \\
        4 & 0.6083 & \textbf{0.7359} \\
        5 & 0.6081 & 0.7018 \\
        \bottomrule
    \end{tabular}
\end{table}


\section{Runtime Analysis}
% - Clarify runtime breakdown in Table 1. Define how time is measured for each method. Clarify what it means by reconstruction (3D reconstruction or feature reconstruction) for each method. Adding VRAM usage for table 1 and table 2
3D open-vocabulary instance segmentation has evolved from traditional 3D object recognition and semantic segmentation, incorporating vision-language models and multi-view scene representations to handle arbitrary object categories \cite{zhu_scanreason_2024, he_segpoint_2024, bhalgat_n2f2_2024, nguyen_any3dis_2024, huang_segment3d_2023, lee_segment_2024, liang_supergseg_2024, koch_relationfield_2024, lyu_gaga_2024, cen_segment_2024, kang_robin3d_2024, yang_set--mark_2023, koch_open3dsg_2024, linok_beyond_2024, zhu_llava-3d_2024, kim_garfield_2024, hu_pointmap_2025, kareem_paris3d_2024}. To assess the practical efficiency of open-vocabulary 3D instance segmentation pipelines, we conduct a detailed runtime analysis of our method and compare it with existing open-vocabulary 3D instance segmentation pipelines on the LERF-OVS \cite{lerf} benchmark. All experiments are performed on a single NVIDIA A100 40GB GPU.  

We report a runtime breakdown using EfficientTAM~\cite{efficienttam} with a frame budget of $P = 40$. The result in~\Cref{tab:ours-runtime-breakdown} shows that 2D feature extraction in our method is a one-time cost, while 2D localization, tracking, and lifting to 3D are fast per query. Query time is primarily governed by the multi-view propagation stage, which accounts for up to 57.78\% of the total runtime. This analysis reinforces the findings in Table 6 of the main paper: replacing the current high-quality tracking segmentor HQ-SAM 2 \cite{samhq} with a faster, on-device tracking segmentor EfficientTAM \cite{efficienttam} can reduce query time significantly.

Compared to prior approaches (~\Cref{tab:runtime-analysis}), which require long 2D feature extraction and 3D feature training or joint reconstruction, our pipeline avoids expensive 3D training and achieves low per-query latency. The 2D feature extraction time of the intensive-preprocess approaches \cite{langsplat,legaussian,opengaussian,instancegaussian,drsplat} are carefully recorded using the preprocessing script provided by LangSplat~\cite{langsplat}. ~\Cref{tab:feature-storage-vram} further highlights that our method uses the least CLIP feature storage and peak VRAM, making it lightweight, scalable, and efficient for consumer-grade GPUs.


\begin{table*}[t]
\centering
\small
\caption{\textbf{Detailed runtime breakdown of our method across scenes and processing stages.} 
2D Feature Extraction is a one-time preprocessing step (refer to Fig. 1 in the main paper).}
\label{tab:ours-runtime-breakdown}

\begin{tabular}{lc|ccc}
\toprule
Scene &
\stackbox{2D Feature Extraction \\ (minutes)} &
\stackbox{2D Localization \\ (minutes)} &
\stackbox{Tracking \\ (s/query)} &
\stackbox{Lifting to 3D \\ (s/query)} \\
\midrule
figurines      & 2.15 min & 0.23 & 0.54 & 0.1 \\
teatime        & 1.14 min & 0.32 & 0.54 & 0.1 \\
ramen          & 1.50 min & 0.29 & 0.47 & 0.1 \\
waldo kitchen          & 1.29 min & 0.29 & 0.53 & 0.1 \\
\midrule
Average        & 1.52 min & 0.28 & 0.52 & 0.1 \\
\bottomrule
\end{tabular}
\end{table*}


\begin{table}[t!]
\footnotesize
\centering
\caption{\textbf{Runtime analysis for open-vocabulary 3D instance segmentation pipelines on LERF-OVS.} Methods marked with * perform joint 3D scene reconstruction during 3D feature training. All other methods operate on pre-reconstructed 3D scenes, which require a few minutes per scene.}
\resizebox{\columnwidth}{!}{%
\label{tab:runtime-analysis}

\begin{tabular}{lccc}
\toprule
\multirow{2}{*}{Method} 
& \multicolumn{1}{c}{2D Feature/Mask} 
& \multicolumn{1}{c}{Training / Lifting} 
& \multicolumn{1}{c}{Inference} \\
& Extraction (minutes) & (minutes) & (s/query)\\
\midrule
\multicolumn{4}{l}{\footnotesize\textit{Training-based \& Pixel-level}} \\
LERF \cite{lerf}                & -- & 45  & 0.04 \\
LangSplat \cite{langsplat}      & 345.00  & 120  & 0.30 \\
LangSplatV2 \cite{langsplatv2}      & 345.00  & 180 & \textbf{0.01} \\
LEGaussians \cite{legaussian}   & 345.00  & 90  & 0.02 \\

\midrule
\multicolumn{4}{l}{\footnotesize\textit{Training-based \& Point-level}} \\
OpenGaussian \cite{opengaussian} & 345.00  & 60  & 0.25 \\
InstanceGaussian \cite{instancegaussian} & 345.00  & 70*  & 0.25 \\
Gaussian Grouping \cite{gaussiangrouping} & 1.50  & 81* & 0.31 \\
ObjectGS \cite{objectgs}        & 1.50 & 102* & 0.31 \\

\midrule
\multicolumn{4}{l}{\footnotesize\textit{Training-free \& Point-level}} \\
Dr. Splat \cite{drsplat}        & 345.00  & 10  & 0.25 \\
LUDVIG \cite{ludvig}            & 6.00  & 4  & 1.30 \\
\textbf{Ours}                   & \textbf{1.50}  & -- & 0.31 \\

\bottomrule
\end{tabular}}
\end{table}

\begin{table}[t]
\centering
\caption{Preprocessing CLIP feature storage (GB) and peak VRAM usage (GB) for open-vocabulary 3D instance segmentation methods on the LERF-OVS benchmark.}
\resizebox{\columnwidth}{!}{%
\label{tab:feature-storage-vram}
\vspace{3pt}
\begin{tabular}{lcc}
\toprule
Method & Feature Storage & Peak VRAM \\
\midrule
LERF \cite{lerf}                & -- & 20 \\
LangSplat \cite{langsplat}      & 2.25 & 10 \\
LangSplatV2 \cite{langsplatv2}            & 2.25 & 47 \\
LEGaussians \cite{legaussian}   & 2.25 & 23 \\
OpenGaussian \cite{opengaussian} & 2.25 & 20 \\
InstanceGaussian \cite{instancegaussian} & 2.25 & 10 \\
Dr.~Splat \cite{drsplat}        & 2.25 & 24 \\
Gaussian Grouping \cite{gaussiangrouping} & -- & 28 \\
ObjectGS \cite{objectgs}        & -- & 30 \\
LUDVIG \cite{ludvig}            & 1.20 & 9 \\
\midrule
\textbf{Ours}                   & \textbf{0.68} & \textbf{5} \\
\bottomrule
\end{tabular}}
\end{table}


\section{More Quantitative and Qualitative Results}
% - Comprehensive qualitative results for LERF-OVS and 3D-OVS. Visualize larger masks
% - Video results: show main proposed components and video results of our extracted masks to prove view consistency of visibility voting (Submitted in compressed zip file including Supp PDF and MP4 from PPT). 
% For each object mask, show: 
% - case 1: w/o visibility voting, w/ visibility voting
% - case 2: InstanceGaussian, LUDVIG, ObjectGS, ours. Show both easy and hard cases. 

% TODO: provide the following discussion
We provide detailed quantitative results and more qualitative results on LERF-OVS dataset \cite{lerf} (\Cref{tab:lerf-ovs}, \Cref{fig:lerf-ovs-figurines}, \Cref{fig:lerf-ovs-ramen}, \Cref{fig:lerf-ovs-teatime}, \Cref{fig:lerf-ovs-waldo}), 3D-OVS dataset \cite{3dovs} (\Cref{fig:3d-ovs-waldo}), and ScanNet dataset~\cite{scannet} (\Cref{fig:scannet}, \Cref{fig:scannet_fullscene}). 
Our method obtains relevant instance masks with clean boundaries by rendering the 3D instance mask reconstructed using our visibility voting technique. 
Other methods such as GaussianGrouping~\cite{gaussiangrouping} and ObjectGS~\cite{objectgs} relied on rasterization from one-hot representations to render masks from the Gaussians, which is less efficient as these methods require to store one-hot features including all object IDs for gaussian and pixel classification. Our voting and rendering mechanism achieves higher visual quality while remaining computationally lightweight, as described in Section 3.3 in the main paper. Unlike pixel-classification-based methods \cite{gaussiangrouping, objectgs}, our voting approach does not require an additional classifier, reducing overhead and simplifying the pipeline.

For instance-aware scene reconstruction methods \cite{gaussiangrouping, objectgs} that do not associate language features with 3D primitives, we enable fair CLIP-based evaluation for the open-vocabulary 3D segmentation task as follows. First, we render all proposed instances in all test views and extract CLIP image features for each rendering of each instance. For each text query, we extract the corresponding CLIP text embedding and compute the cosine similarity between the query embedding and each instance’s CLIP image feature. We then select the instance whose rendering yields the highest similarity score to the prompted text. Finally, the masks of the chosen instances in the test views are evaluated against the ground-truth instance masks.

For LUGVIG~\cite{ludvig}, the original method does not provide implementation to extract 3D Gaussians for each instance for mask rendering.
We evaluate instance segmentation performance using the provided diffusion masks, and exclude SAM refinement to ensure fair comparison of instance rendering quality. Qualitative visualizations are generated by showing only the rendered pixels that fall within each instance mask.

\begin{table*}[ht!]
\centering
\caption{Open-vocabulary 3D instance segmentation results on LERF-OVS \cite{lerf}.}
\resizebox{\textwidth}{!}{%
\label{tab:lerf-ovs}
\begin{tabular}{lccccccccccc}
\toprule
\multirow{2}{*}{Method} & \multicolumn{5}{c}{mIoU $\uparrow$} & \multicolumn{5}{c}{mAcc@0.25 $\uparrow$} & \multirow{2}{*}{TTFQ $\downarrow$} \\
\cmidrule(lr){2-6} \cmidrule(lr){7-11}
 & figurines & teatime & ramen & waldo & mean & figurines & teatime & ramen & waldo & mean &  \\
\midrule
\multicolumn{12}{l}{\textit{Training-based \& Pixel-level}} \\
LERF \cite{lerf} & 38.60 & 45.00 & 28.40 & 37.90 & 37.48 & 75.00 & 84.80 & 75.00 & 72.70 & 76.88 & 34 min \\
LangSplat \cite{langsplat} & 44.70 & 58.48 & 49.33 & 34.48 & 46.75 & 73.21 & 79.66 & 60.56 & 59.09 & 68.13 & 7 hours \\
LEGaussians \cite{legaussian} & 40.80 & 60.30 & \underline{46.00} & 39.40 & 46.63 & 75.00 & 64.46 & 51.25 & 48.91 & 59.91 & 7 hours \\
LangSplatV2 \cite{langsplatv2} & 56.40 & 72.20 & 51.80 & 59.10 & \underline{59.90} & \underline{82.10} & \textbf{93.20} & 74.70 & \textbf{86.40} & \underline{84.10} & 10 hours \\
\midrule
\multicolumn{12}{l}{\textit{Training-based \& Point-level}} \\
OpenGaussian \cite{opengaussian} & 39.29 & 60.44 & 31.01 & 22.70 & 38.36 & 55.36 & 76.27 & 42.25 & 31.82 & 51.43 & 7 hours \\
InstanceGaussian \cite{instancegaussian} & 47.92 & 60.34 & 29.73 & 36.52 & 43.63 & 66.07 & 79.66 & 46.47 & 59.09 & 62.82 & 7 hours \\
Gaussian Grouping \cite{gaussiangrouping} & 47.99 & \underline{74.63} & 34.67 & 15.35 & 43.16 & 51.78 & 84.74 & 47.88 & 18.18 & 50.65 & 1 hours \\
ObjectGS \cite{objectgs} & \underline{66.03} & 67.90 & 44.59 & 21.81 & 50.08 & 76.78 & 77.96 & 60.56 & 27.27 & 60.64 & 2 hours \\
Segment-then-Splat \cite{segmentthensplat} & -- & -- & -- & -- & 52.10 & -- & -- & -- & -- & -- & 2 hours \\
\midrule
\multicolumn{12}{l}{\textit{Training-free \& Point-level}} \\
Dr. Splat \cite{drsplat} & 53.36 & 57.20 & 24.70 & 39.07 & 43.58 & 63.64 & 35.21 & \textbf{80.36} & 76.27 & 63.87 & 6 hours \\
LUDVIG \cite{ludvig} & 58.03 & 59.77 & 42.31 & \underline{42.19} & 50.58 & 71.42 & 59.77 & 69.01 & 42.19 & 60.59 & 10 min \\
Ours & \textbf{72.98} & \textbf{74.76} & \textbf{59.80} & \textbf{44.54} & \textbf{63.02} & \textbf{96.43} & \underline{84.80} & \underline{76.23} & \underline{82.18} & \textbf{84.91} & \textbf{1.5 min} \\
\bottomrule
\end{tabular}}
% \vspace{-20pt}
\end{table*}

\begin{figure*}[t!]
    \centering
    \includegraphics[width=\linewidth]{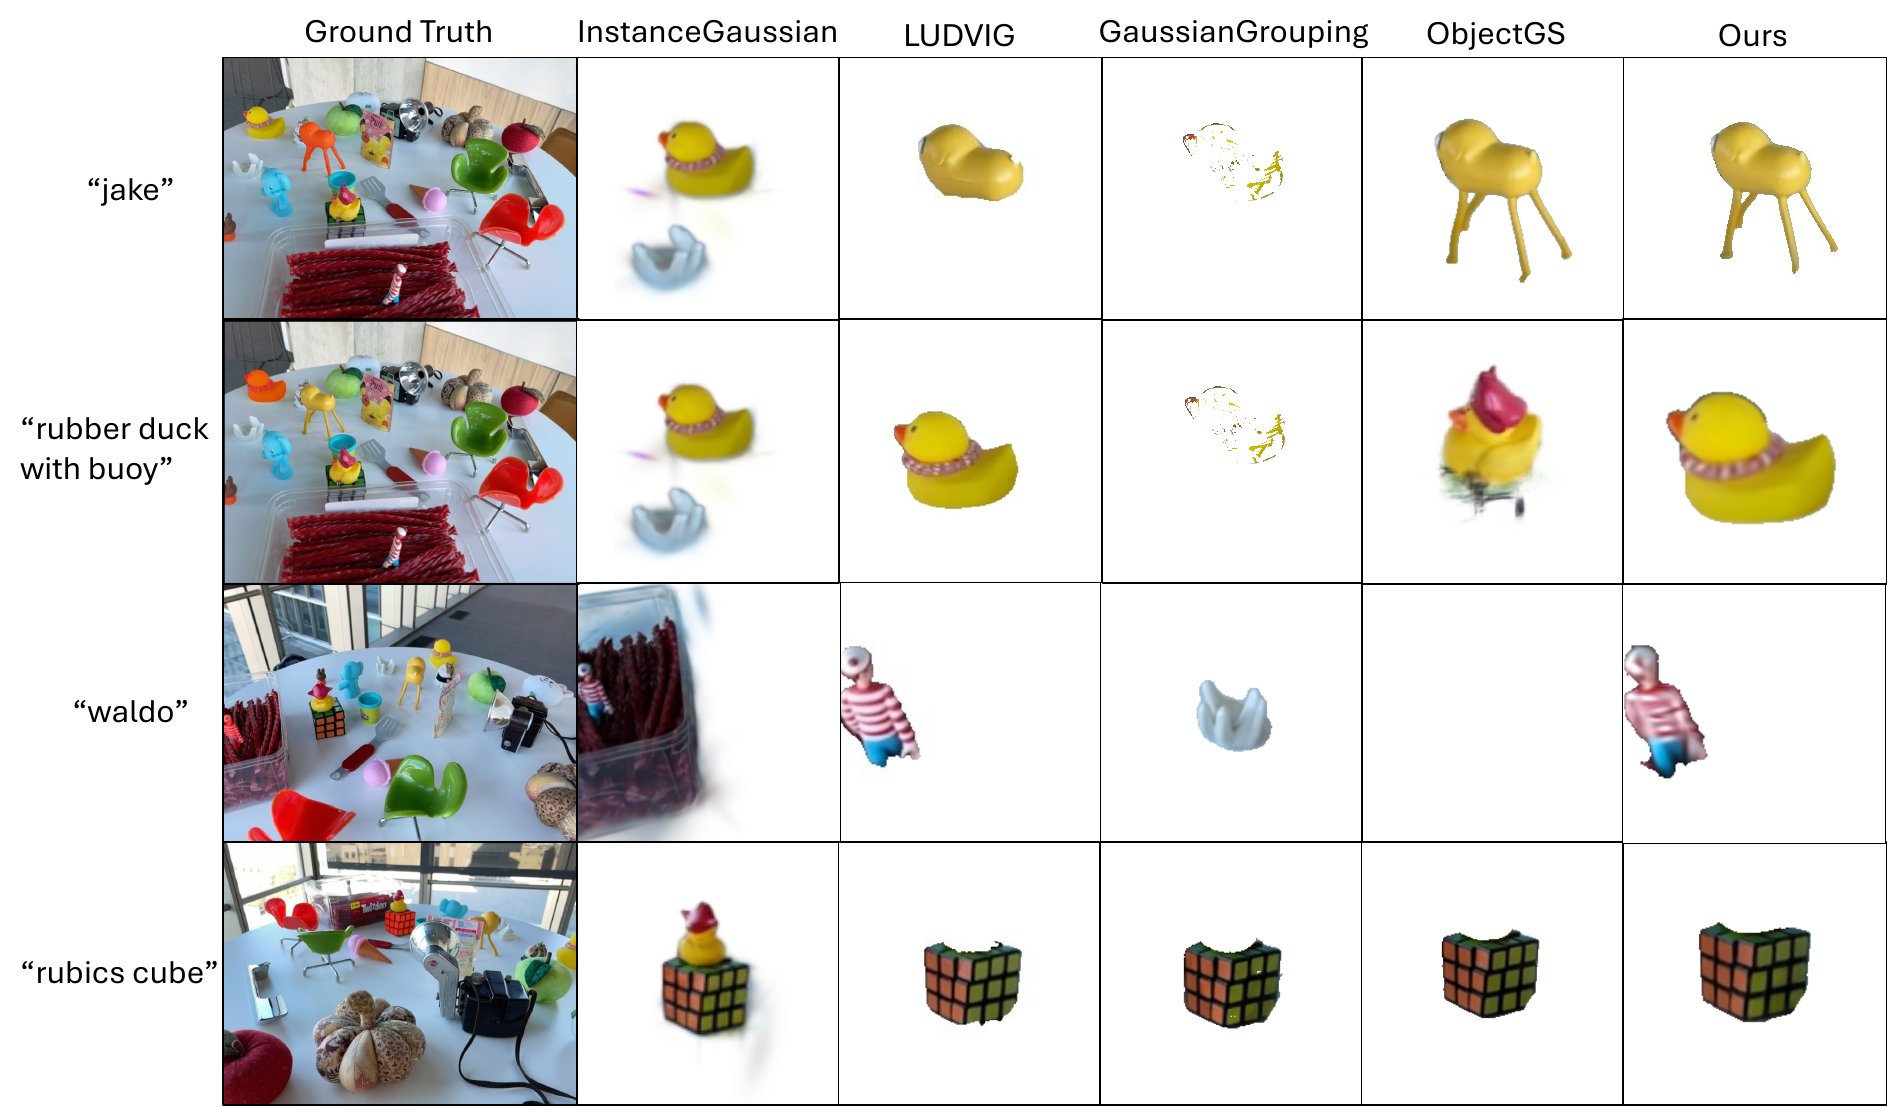}
    \vspace{-5pt}
    \caption{
    Qualitative comparison on scene Figurines of LERF-OVS benchmark.
    }
    \vspace{-10pt}
    \label{fig:lerf-ovs-figurines}
\end{figure*}

\begin{figure*}[t!]
    \centering
    \includegraphics[width=\linewidth]{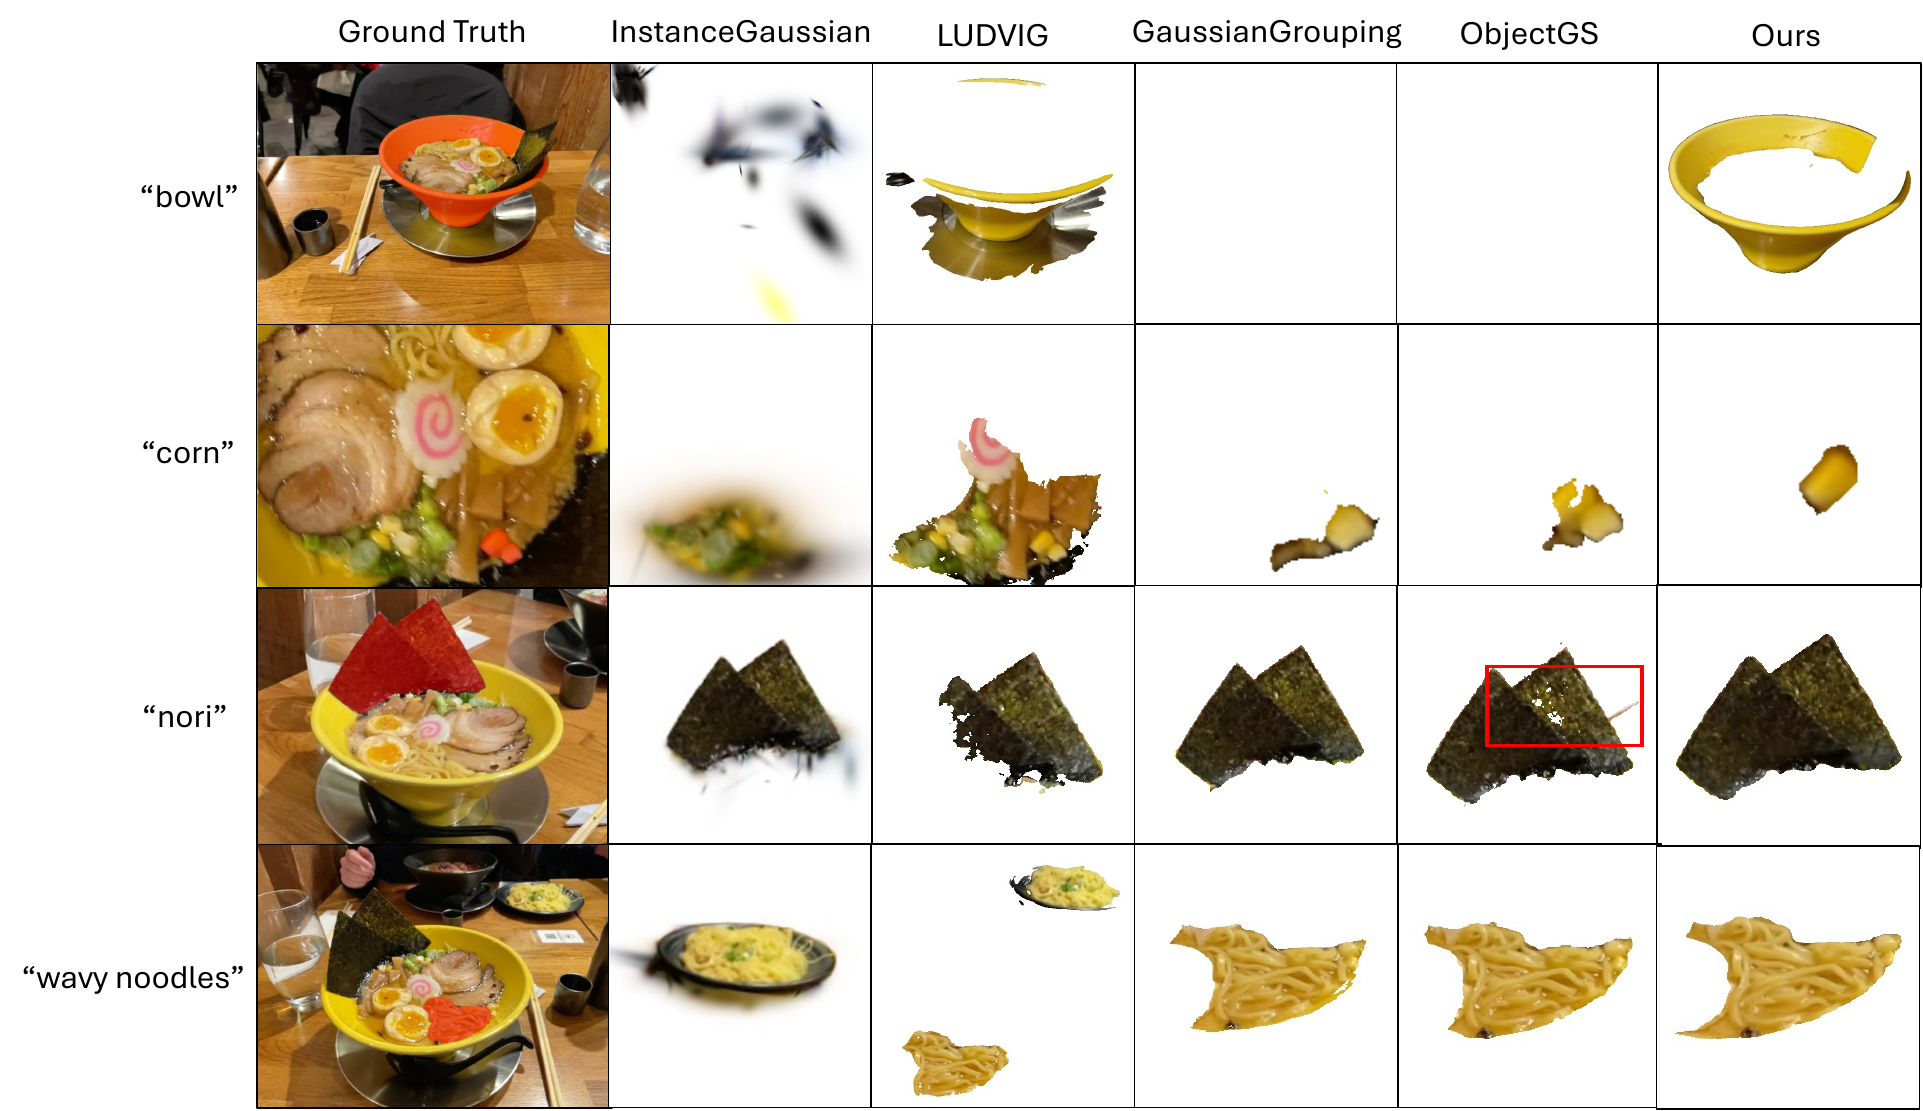}
    \vspace{-5pt}
    \caption{
    Qualitative comparison on scene Ramen of LERF-OVS benchmark.
    }
    \vspace{-10pt}
    \label{fig:lerf-ovs-ramen}
\end{figure*}

\begin{figure*}[t!]
    \centering
    \includegraphics[width=\linewidth]{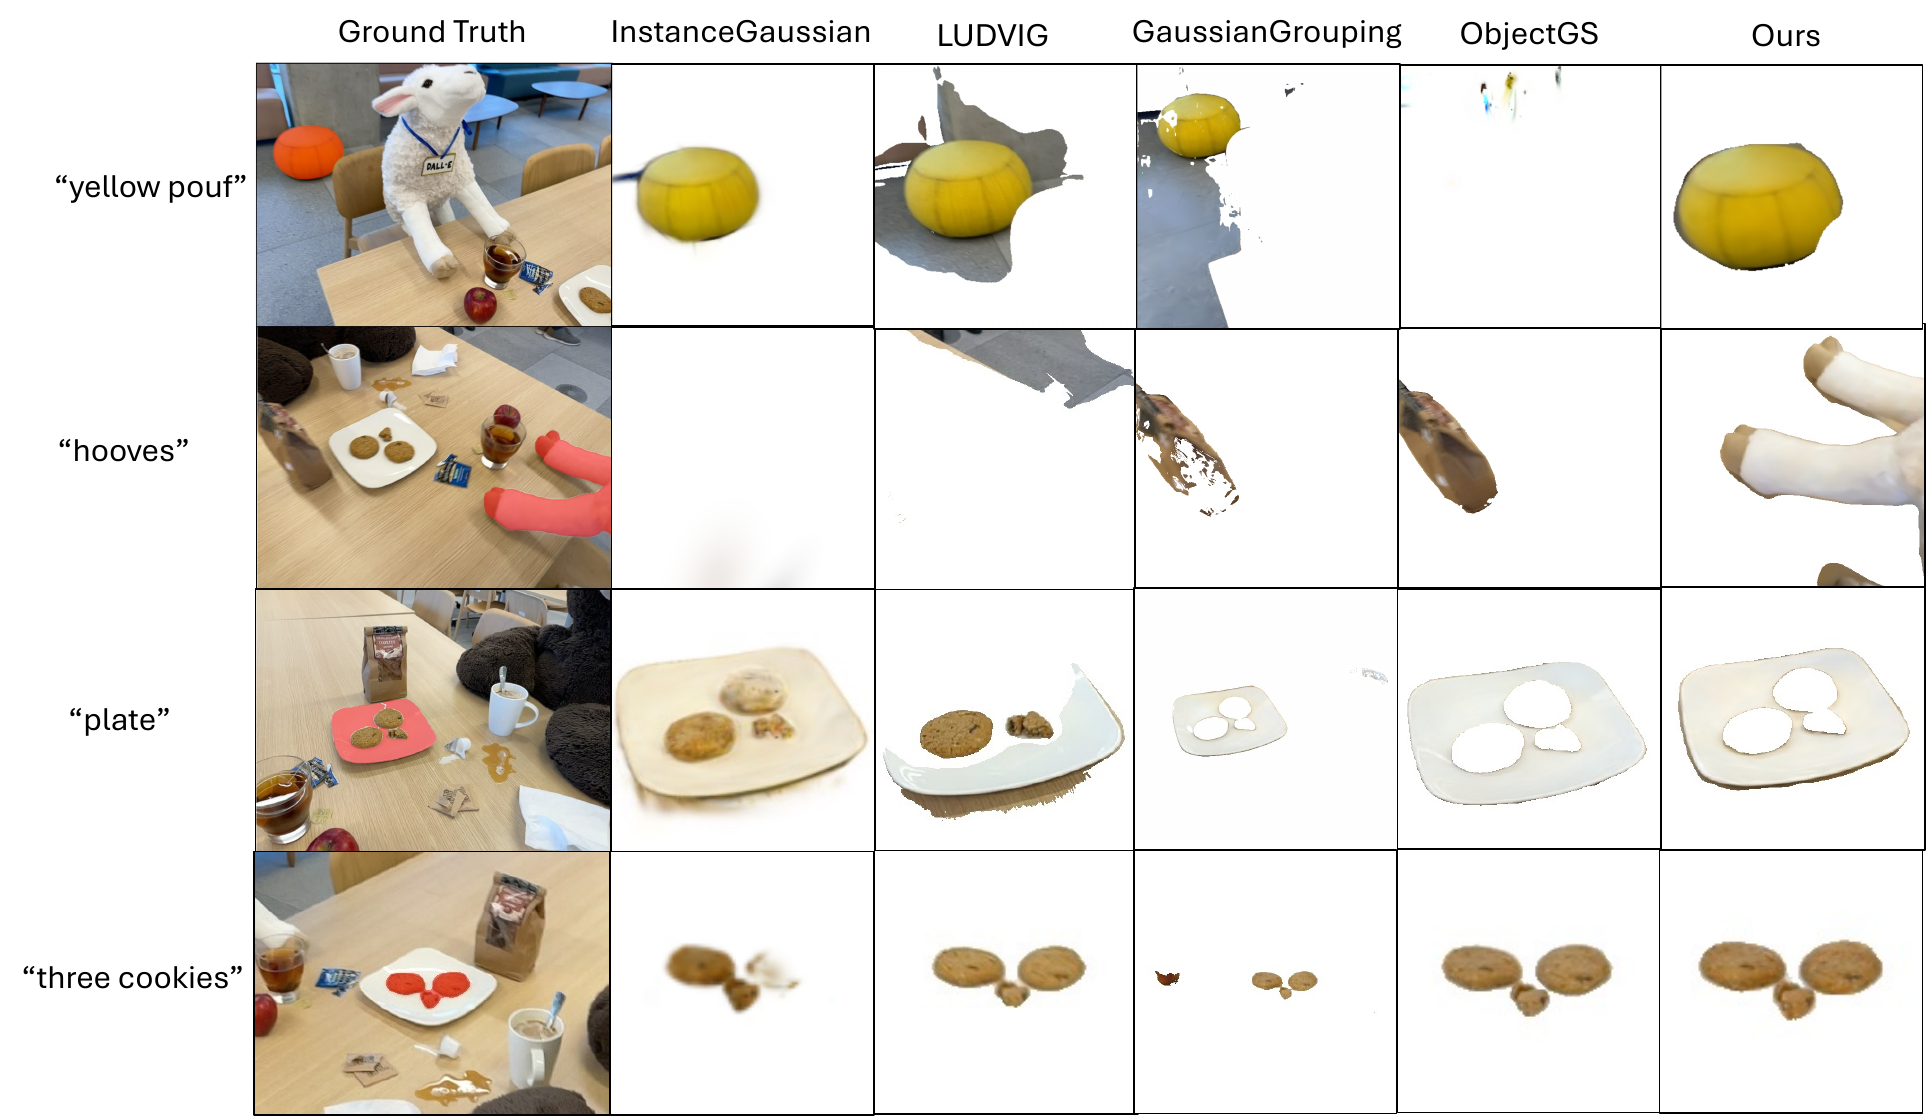}
    \vspace{-5pt}
    \caption{
    Qualitative comparison on scene Teatime of LERF-OVS benchmark.
    }
    \vspace{-10pt}
    \label{fig:lerf-ovs-teatime}
\end{figure*}

\begin{figure*}[t!]
    \centering
    \includegraphics[width=\linewidth]{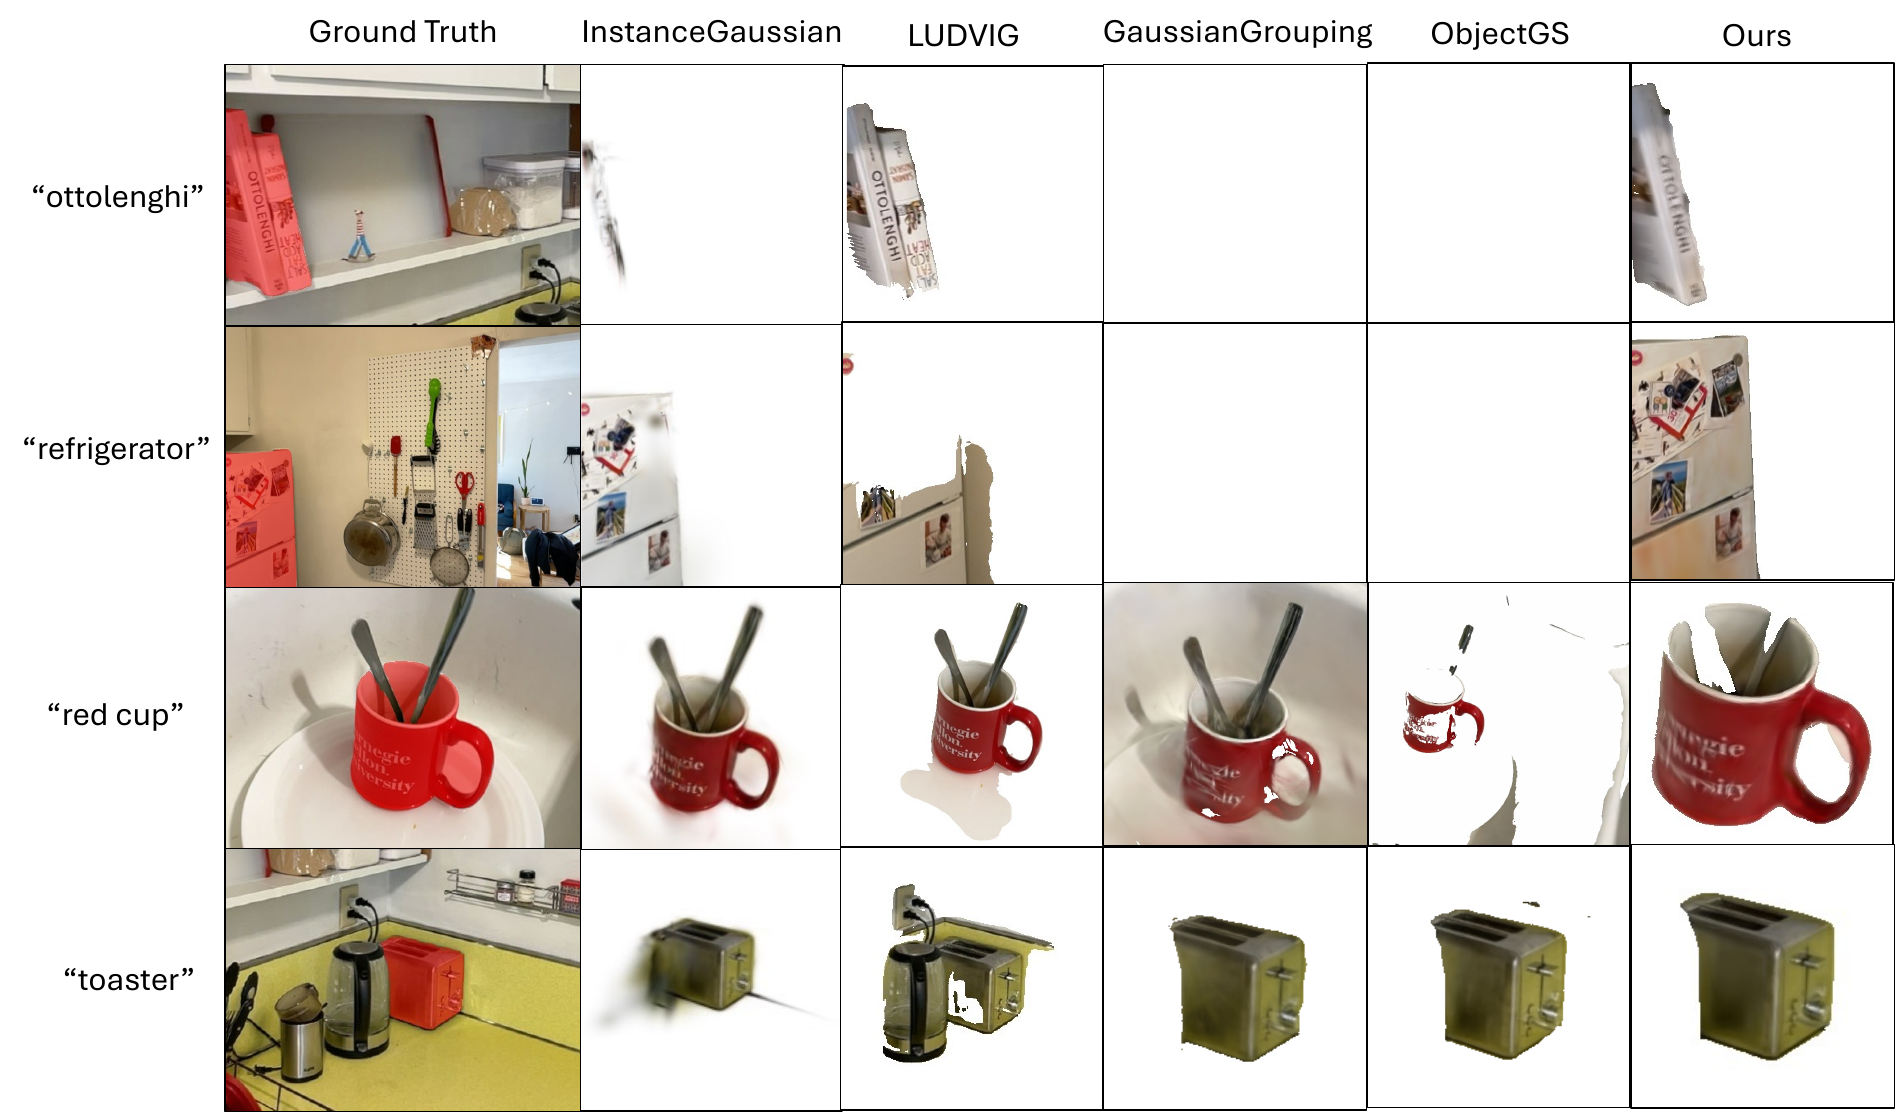}
    \vspace{-5pt}
    \caption{
    Qualitative comparison on scene Waldo Kitchen of LERF-OVS benchmark.
    }
    \vspace{-10pt}
    \label{fig:lerf-ovs-waldo}
\end{figure*}

\begin{figure*}[t!]
    \centering
    \includegraphics[width=\linewidth]{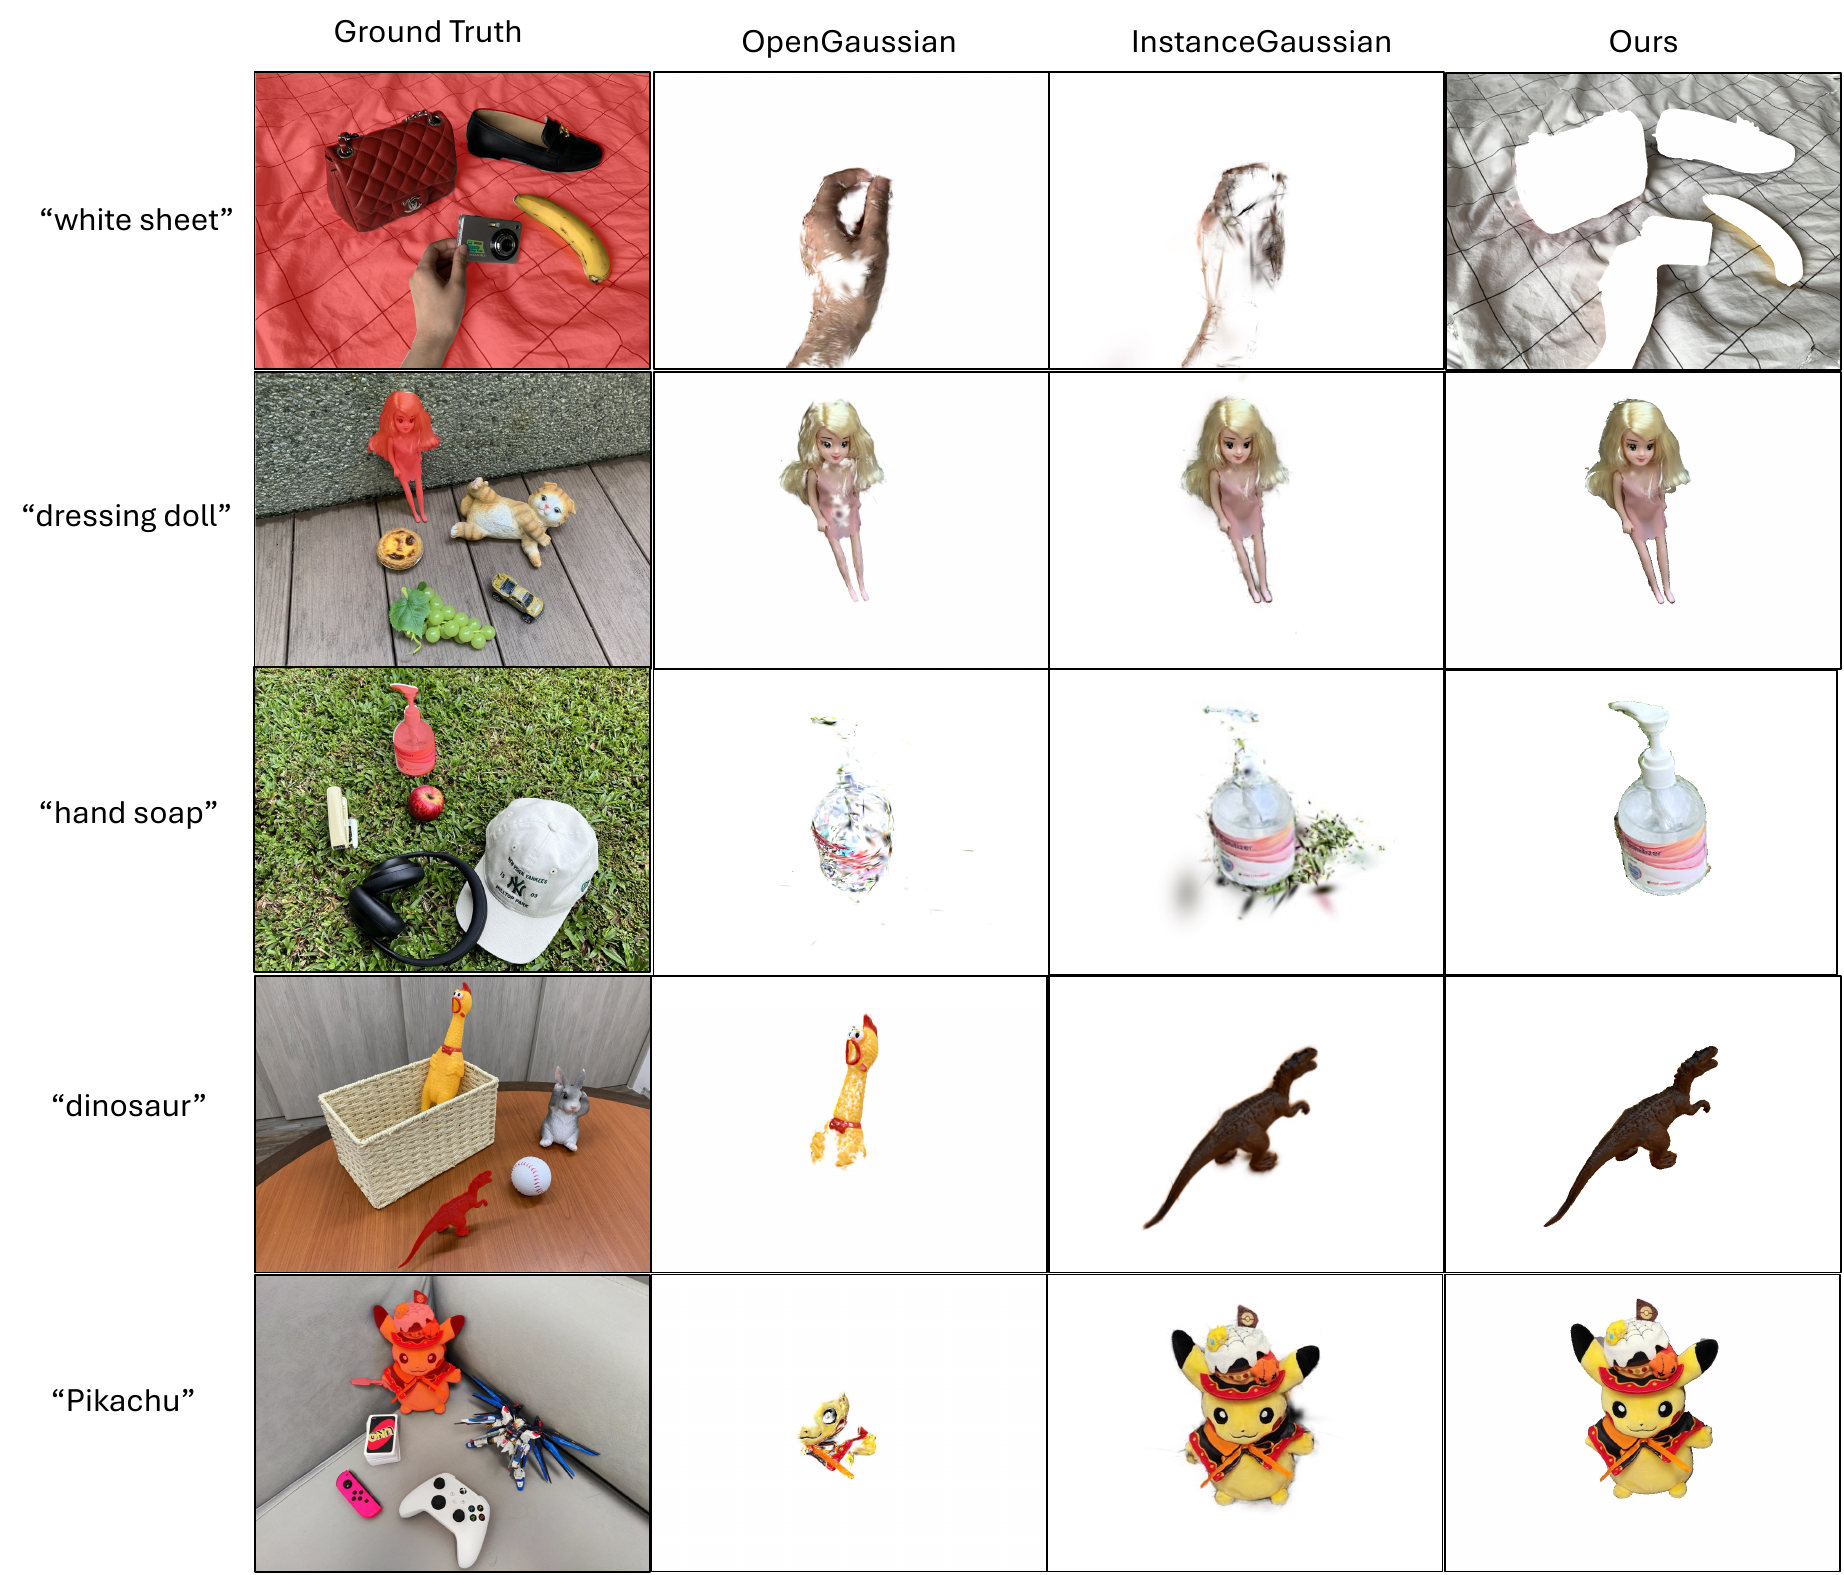}
    \vspace{-5pt}
    \caption{
    Qualitative comparison on 3D-OVS benchmark.
    }
    \vspace{-10pt}
    \label{fig:3d-ovs-waldo}
\end{figure*}

\begin{figure*}[t!]
    \centering
    \includegraphics[width=\linewidth]{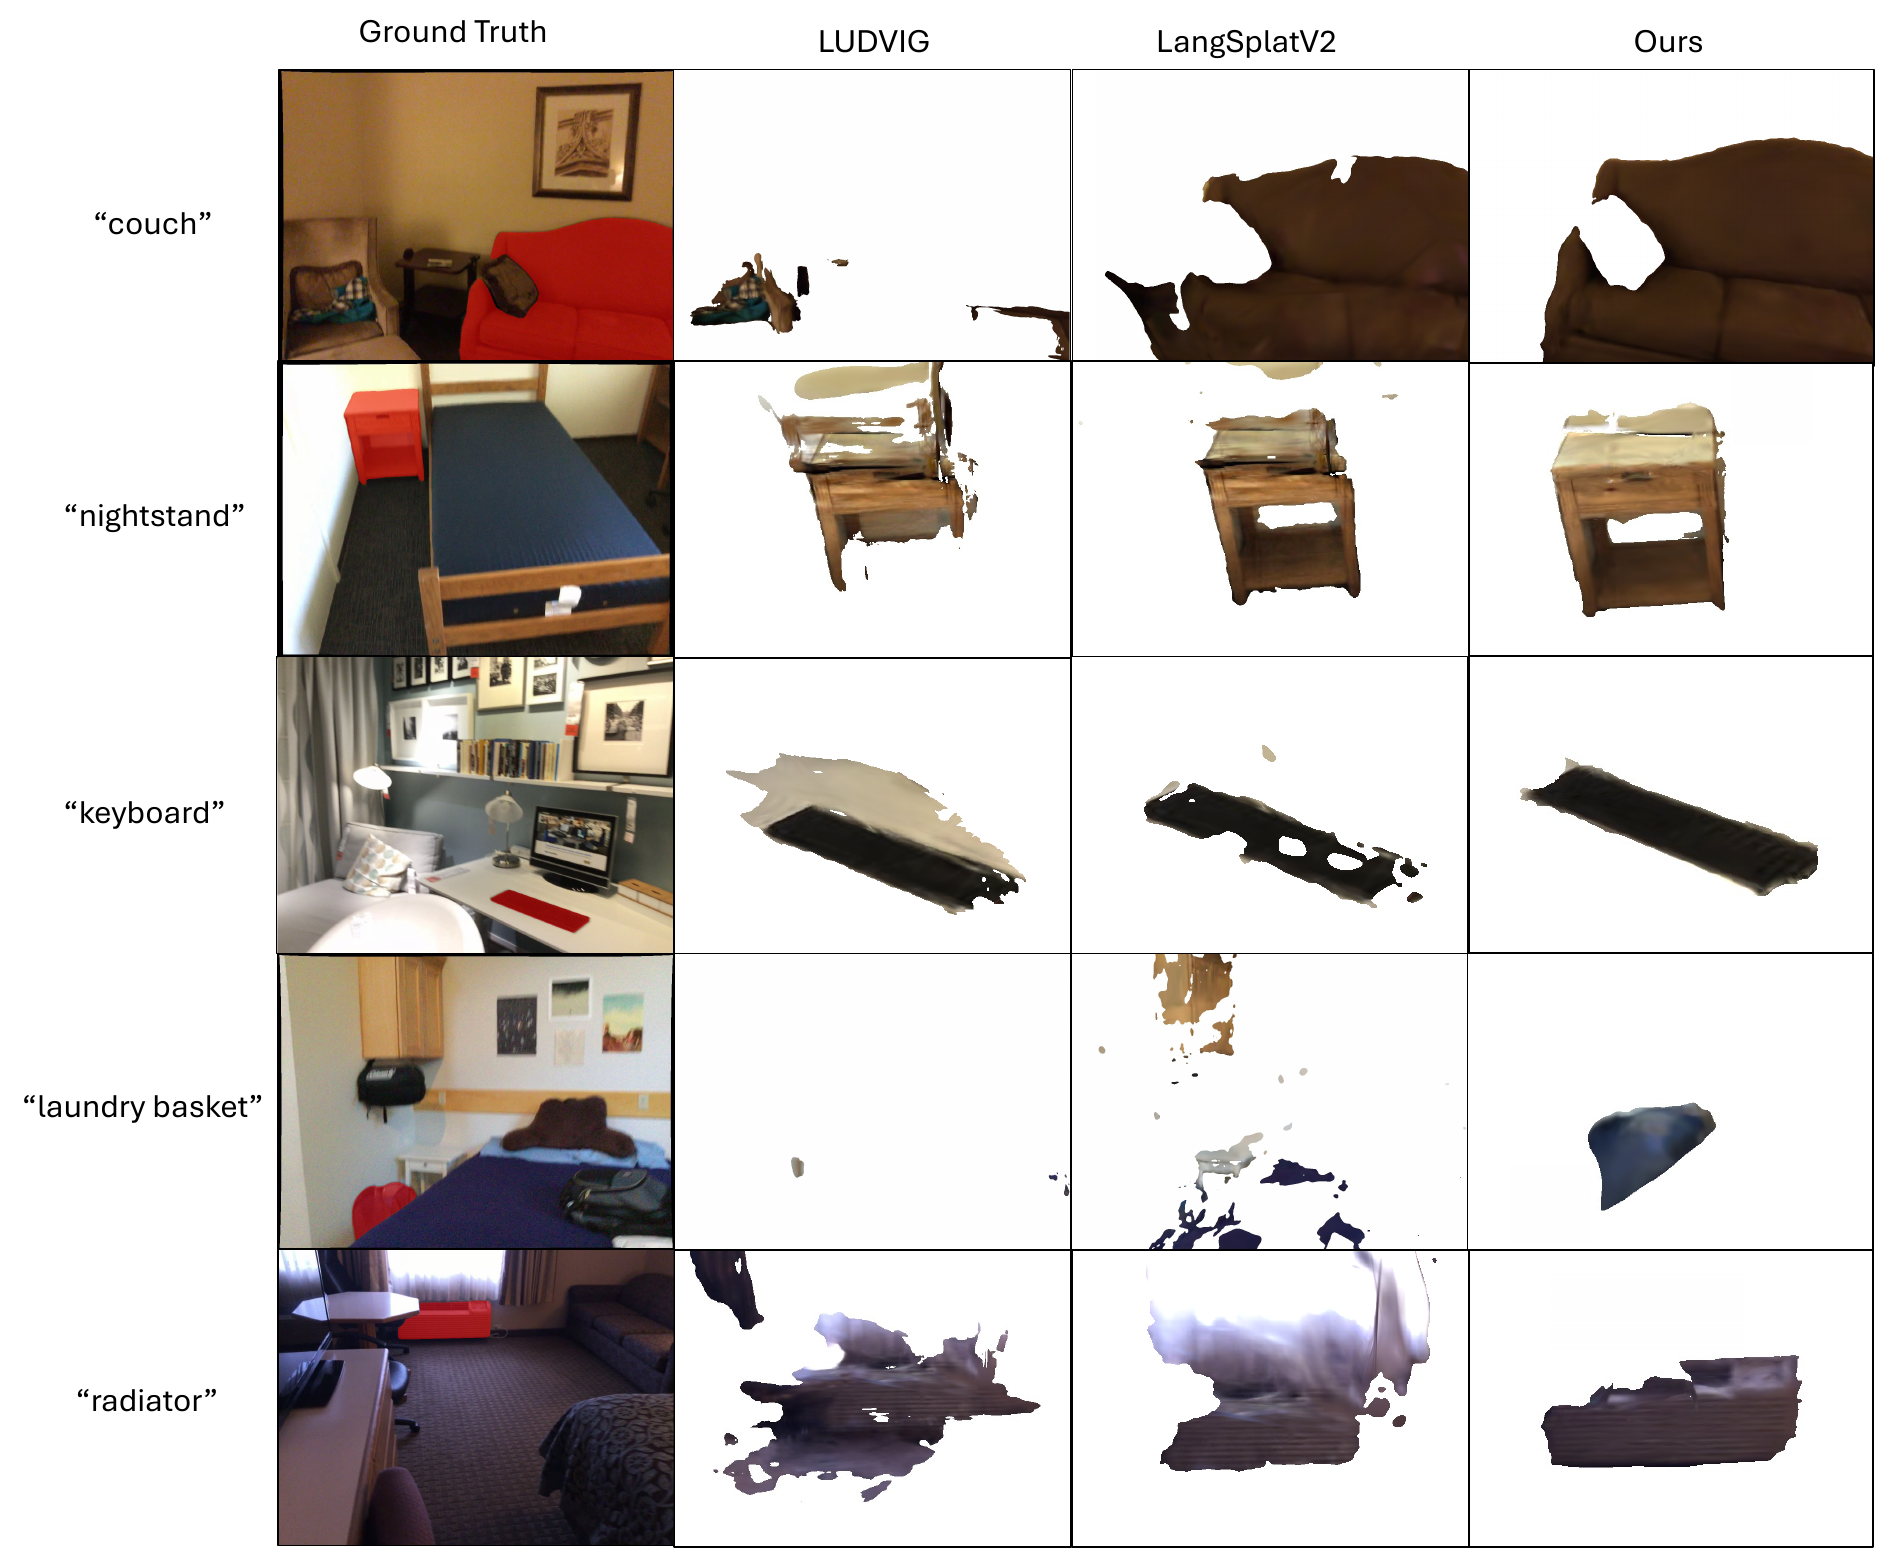}
    \vspace{-5pt}
    \caption{
    Qualitative comparison on ScanNet benchmark.
    }
    \vspace{-10pt}
    \label{fig:scannet}
\end{figure*}

\begin{figure*}[t]
    \centering
  \includegraphics[width=\linewidth]{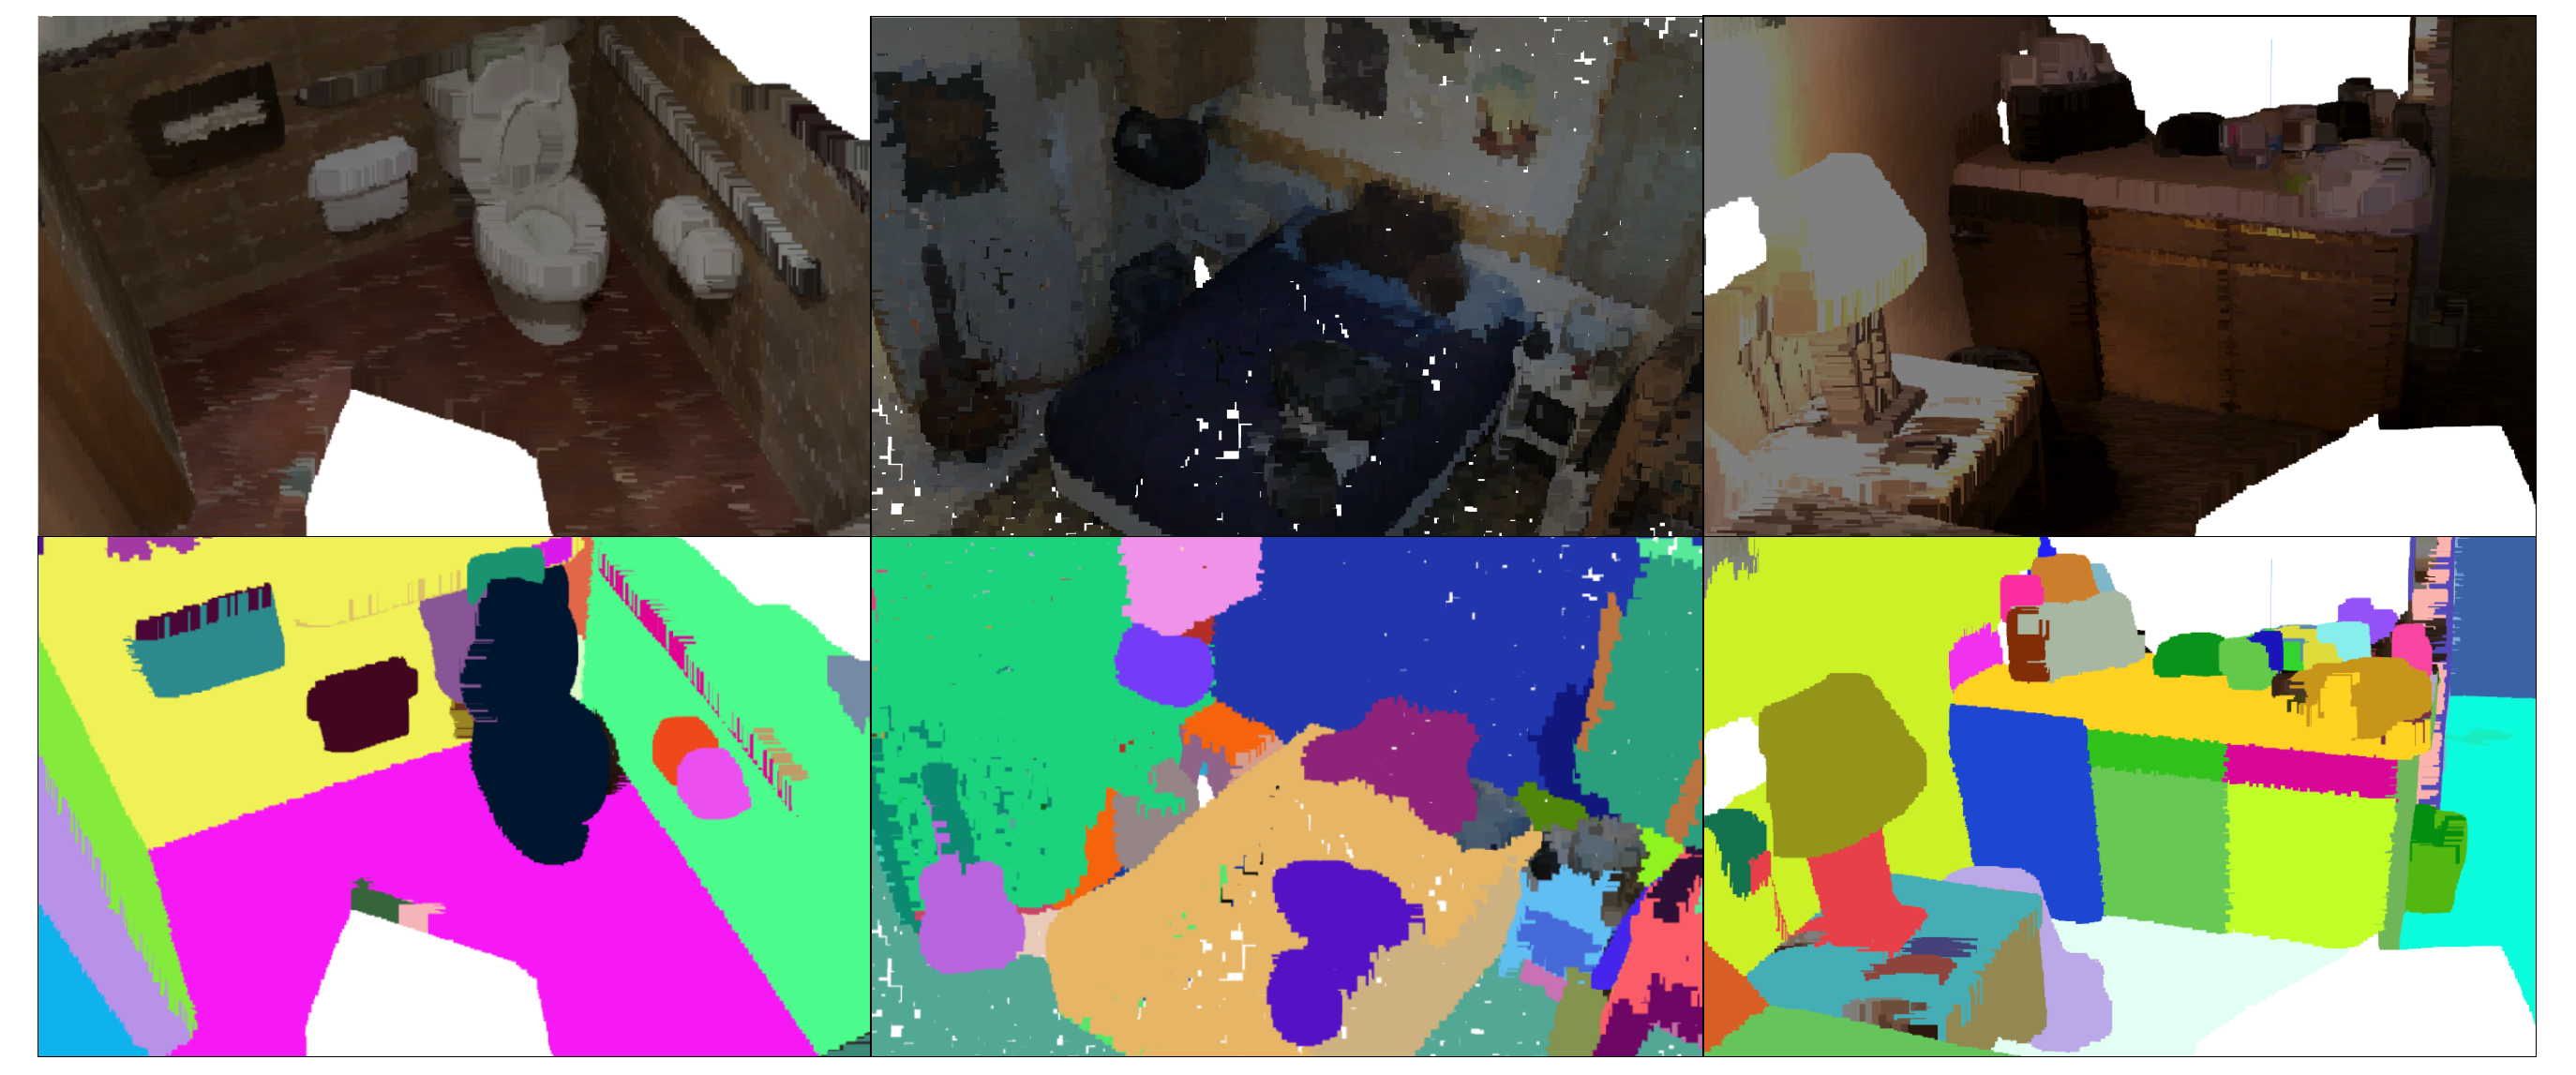}
    \caption{Class-agnostic instance segmentation on ScanNet.}
    \label{fig:scannet_fullscene}
\end{figure*}
% 
\section{Scalability to Large Scenes}
Regarding scalability, the only additional cost in larger scenes arises during preprocessing, where dense CLIP features are extracted for each image (0.75 seconds per image), which scales linearly with the number of frames. The downstream stages, namely tracking, propagation, and visibility voting, operate under a fixed frame budget and do not grow with scene size.

\section{Limitations and Future Works}
While our method is designed for efficient query-wise open-vocabulary 3D instance segmentation, several limitations remain. First, tracking quality can degrade under large viewpoint changes, leading to drift during multi-view propagation. Although our mask refinement module alleviates this issue, more robust long-range correspondence mechanisms could further improve performance. Second, severe occlusions may result in incomplete 3D masks. Our visibility voting strategy mitigates this problem by aggregating evidence across views, but it cannot fully recover regions that are consistently occluded. Moreover, performance on ambiguous queries is bounded by the semantic reasoning capability of the underlying CLIP model. Although iterative multi-instance suppression helps distinguish multiple candidate instances, inaccurate or ambiguous vision-language alignment can still lead to localization errors. Besides, our budget-aware view selection may provide insufficient coverage for highly elongated or heavily occluded objects, particularly when their geometry spans complex layouts. Although $P$ is configurable to allow more propagated views, more adaptive view budgeting could further improve 3D mask completeness in such challenging cases. Finally, when adjacent instances have highly similar appearances and no visible gap, the boundary stopping criterion may fail to fully separate them, potentially causing mask leakage. As shown in Fig.~\ref{fig:adjacent_query}, our method effectively separates adjacent instances when a visible gap is present, while directly adjacent instances with similar appearances remain challenging.

\begin{figure}[H]
    \centering
    \includegraphics[width=\linewidth]{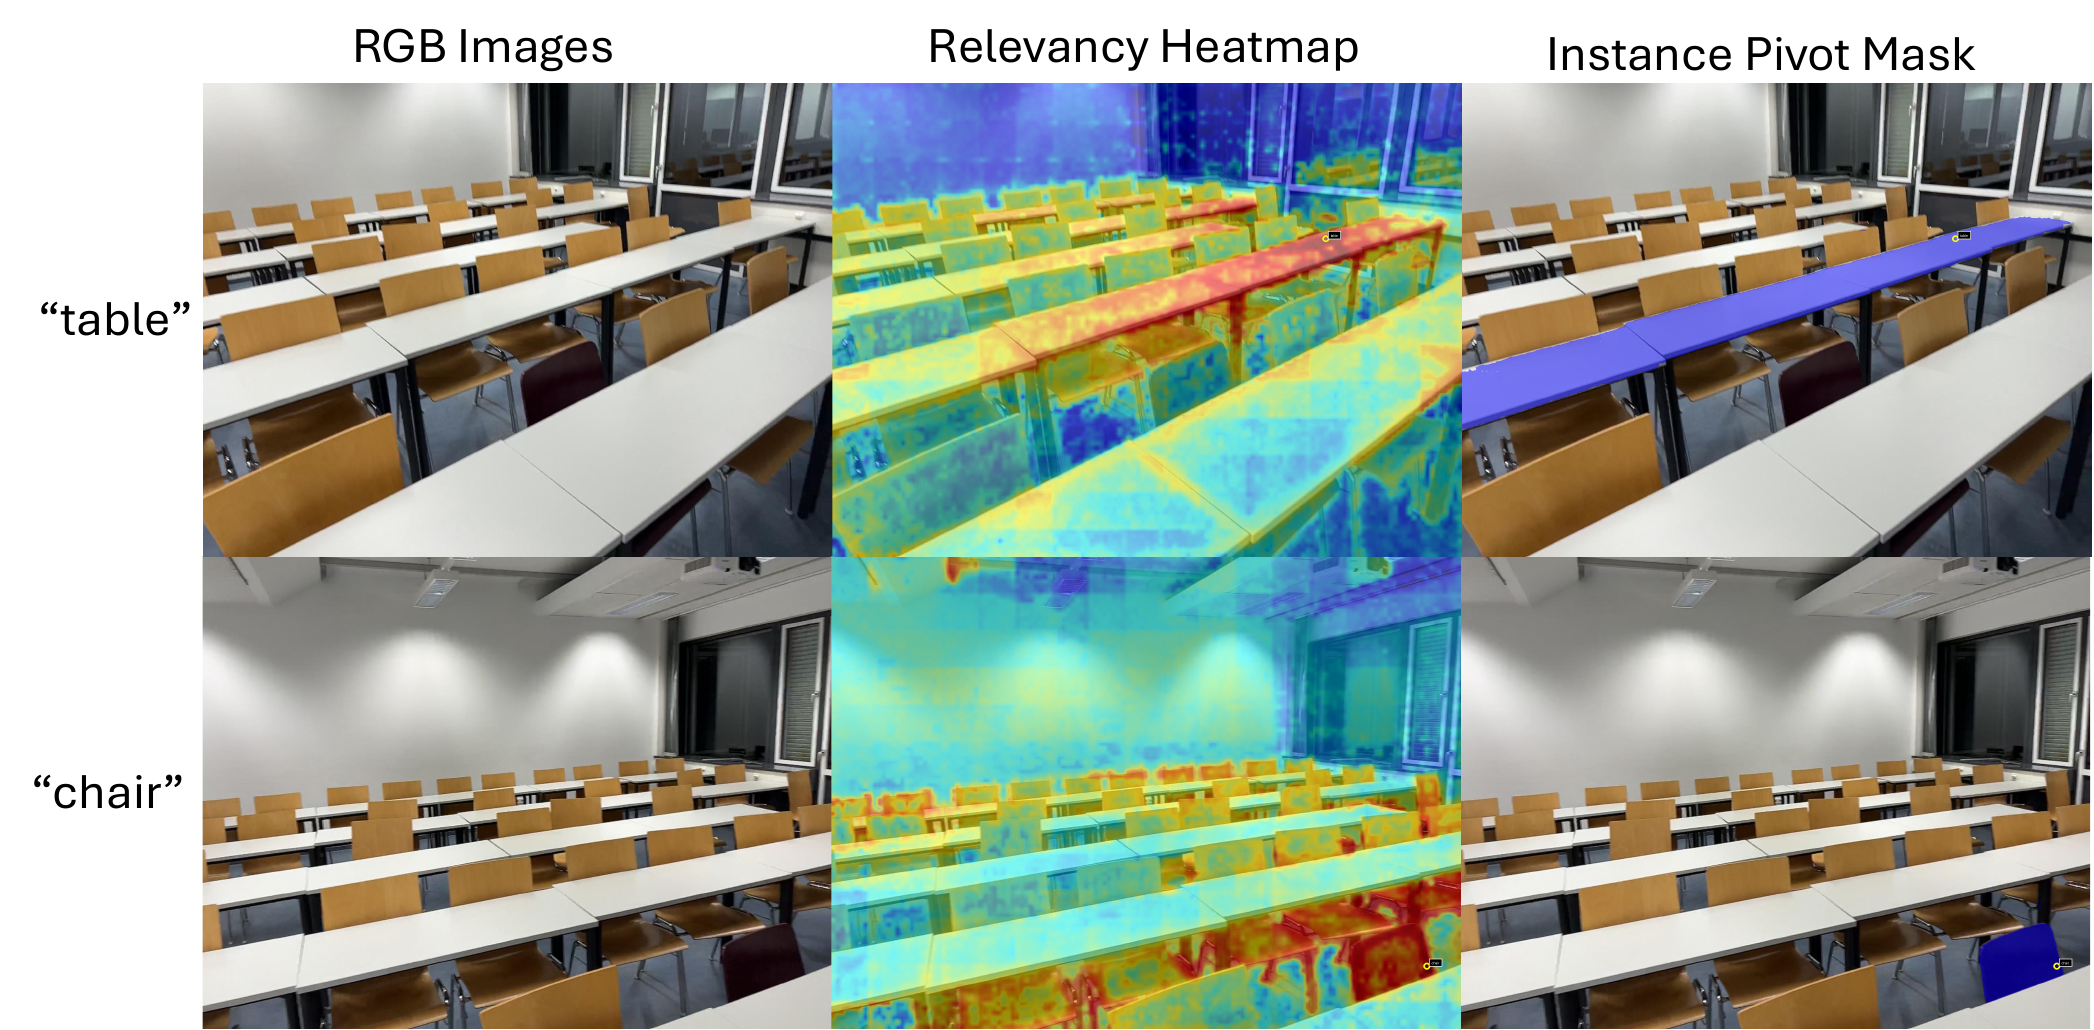}
    \caption{Limitation of the boundary stopping criterion on adjacent instances with invisible gaps.}
    \label{fig:adjacent_query}
\end{figure}


From an efficiency perspective, future work could further reduce dense CLIP feature extraction latency, improve the robustness of the tracking process, and develop comprehensive benchmarks for evaluating object parts, sub-parts, and multiple instances under challenging conditions. In addition, our method is primarily designed for object-centric queries. Although it performs well on small and fine-grained objects (e.g., the \emph{pirate hat} example in Fig. 3 of the main paper), extending the framework to support large structural regions such as walls, floors, and other scene-level elements remains an important direction for future research. Finally, incorporating model compression and quantization techniques would facilitate deployment on resource-constrained and edge devices.

\section{Details of Evaluation Benchmarks}
We evaluate our method on four standard open-vocabulary 3D instance segmentation benchmarks: LERF-OVS~\cite{lerf}, 3D-OVS~\cite{3dovs}, ScanNet~\cite{scannet}, and ScanNet++~\cite{scannetpp}, all of which are widely used by prior approaches for benchmarking open-vocabulary 3D scene understanding \cite{drsplat,opengaussian,instancegaussian,langsplat,legaussian, opensplat3d}. We adopt the standard train/test splits for all datasets.
 
LERF-OVS contains four indoor scenes with complex geometry and 100–300 multi-view RGB images covering 360°, along with ground-truth 2D instance masks for 10–20 short-text queries. The queries cover diverse cases, including small instances, groups of instances, and object parts, with text ranging from generic nouns to specific object names and categories such as toys, food, and kitchen objects.

3D-OVS includes five indoor and outdoor scenes with 60–120 front-facing images, covering diverse settings, including indoor environments and low-quality images. The scenes contain both simple and structurally complex query objects, including long-tail objects in varied poses and backgrounds. Ground-truth masks for the test views are manually annotated.

 We follow prior work~\cite{opengaussian,instancegaussian} and benchmark on 10 randomly selected ScanNet scenes. ScanNet is an RGB-D video dataset, annotated with 3D camera poses, surface reconstructions, and instance-level semantic segmentations. To evaluate performance in large-scale and cluttered environments, we further provide new 2D segmentation annotations covering 63 categories to evaluate unique-instance localization in densely cluttered scenes. 
 
 In addition, we evaluate class-agnostic 3D instance segmentation on the full ScanNet++ validation split (50 scenes) following the Open3DIS protocol. Collectively, these benchmarks assess generalization across diverse scene types, varying geometric complexity, short and compositional queries, and both complete and partial scene coverage. 
